# Supplementary material for: A Renormalization Group Approach to Connect Discrete- and Continuous-Time Descriptions of Gaussian Processes
Source: arXiv:2101.06482 source file (2021-12-07)
Supplement: Supplementary file 1 [file si_old.tex]

\section*{SUPPLEMENTAL MATERIAL:\\
The Connection Between Discrete- and Continuous-Time Descriptions of Gaussian Continuous Processes}
%
\author{Federica Ferretti}
%\email{f.ferretti@uniroma1.it}
\author{Victor Chard\`es}
%\email{chardes@lpt.ens.fr}
\author{Thierry Mora}
\author{Aleksandra M Walczak}
%\email{awalczak@lpt.ens.fr}
\author{Irene Giardina}

%\maketitle
\renewcommand{\theequation}{S\arabic{equation}}
\renewcommand{\thefigure}{S\arabic{figure}}
\renewcommand{\thetable}{S\arabic{table}}
\setcounter{equation}{0}
\setcounter{table}{0}
\setcounter{figure}{0}

%\tableofcontents

%%%%%%%%%%%%%%%%%%%%%%%%%%%%%%%%%%%%%%%%%%%%%%%%%%%%%%%%%%%%%%
%%%%%%%%%%%%%%%%%%%%%%%%%%%%%%%%%%%%%%%%%%%%%%%%%%%%%%%%%%%%%%
\section*{I. Decimation of general ARMA($p,q$) models}

An autoregressive moving-average process of order $(p,q)$, denoted ARMA($p,q$), is a time series generated by the update equation
\begin{equation}
X_n = \sum_{i=1}^p\phi_iX_{n-i} +\sum_{i=1}^q \nu_i \epsilon_{n-i} + \mu\epsilon_n
\label{arma-pq-def}
\end{equation}
with $\epsilon_n\sim \mathcal N(0,1)$ I.I.D., $\nu_i, \mu \in \mathbb R$. The autoregressive (AR) part of the equation, of order $p$, can be thought of as the discretization of the deterministic part of an associated continuous-time dynamical model, and corresponds to the first RHS sum of Eq.~\eqref{arma-pq-def}. The moving average (MA) part, of order $q$, corresponds to the second RHS sum of Eq.~\eqref{arma-pq-def}. For the sake of simplicity, we rename the whole random increment as $r_n = \sum_{i=1}^q \nu_i \epsilon_{n-i} + \mu\epsilon_n$. We show in this section that, given a general ARMA($p,q$) model, there must exist a specific relation between $p$ and $q$ if the property of invariance under coarse-graining is required. 

We apply to autoregressive time-series models a Renormalization Group (RG) procedure inspired to real space renormalization of one-dimensional spin chains. In this analogy, discretely observed states of the system play the role of spin variables sitting on lattice sites, and time steps correspond to lattice spacings. Each RG iteration consists of two operations:
\begin{enumerate}
\item coarse-graining by decimation, i.e. we derive the update equations for the subseries of even time states;
\item joint rescaling of the time step, $2\tau\to\tau$, and of the parameters of the model, according to their physical dimension.
\end{enumerate}

In the decimation step, we want to trim a point out of two in the time sequence generated by Eq.~\eqref{arma-pq-def}, as sketched in Fig.~\ref{fig:schematic}a. In order to do it, we use the linear combination 
\begin{equation}
\text{Eqn}(X_n) + \sum_{i=1}^p(-1)^{i+1}\phi_i \text{Eqn}(X_{n-i}).
\label{comb-pq}
\end{equation}
Notice that this combination only depends on the AR order $p$. The resulting discrete-time model reads:
\begin{dmath}
X_n = \underbrace{\sum_{i=1}^p\left[1+(-1)^i\right]\phi_iX_{n-i}}_{\encircle{A}} + \underbrace{\sum_{i=1}^p(-1)^{i+1}\phi_i\sum_{k=1}^p\phi_kX_{n-k-i}}_{\encircle B} + \underbrace{\mu_0\epsilon_n+ \sum_{j=1}^q\mu_j\epsilon_{n-j}+\sum_{i=1}^p(-1)^{i+1}\phi_i\left[\mu_0\epsilon_{n-i}+\sum_{k=1}^q\mu_k\epsilon_{n-i-k}\right]}_{\tilde r_n}.
\label{cg-pq}
\end{dmath}
Sum \encircle{B} in Eq.~\eqref{cg-pq} can be rewritten, with a rearrangement of terms, as 
%cast into a recursive structure:
%\begin{dmath}
%\sum_{i=1}^p(-1)^{i+1}\phi_i\sum_{k=1}^p\phi_kX_{n-k-i} = 
%	\phi_1^2X_{n-2}+2\phi_1\sum_{k=1}^{\lfloor\frac{p-1}{2}\rfloor}\phi_{2k+1}X_{n-2-2k} + \sum_{i=2}^p (-1)^{i+1}\phi_i\sum_{k=2}^p\phi_kX_{n-k-i}, 
%\label{eq:cast}
%\end{dmath}
%as the last term in Eq.~\eqref{eq:cast} can be rewritten as $-\sum_{i=1}^{p-1} (-1)^{i+1}\phi_{i+1}\sum_{k=1}^{p-1}\phi_{k+1}X_{n-2-k-i}$ and the same decomposition used to derive Eq.~\eqref{eq:cast} can be repeatedly applied. As a result:
\begin{equation}
{\encircle B} = \sum_{i=1}^p(-1)^{i+1}\phi_i\sum_{k=1}^p\phi_kX_{n-k-i} = \sum_{i=1}^p(-1)^{i+1}\left(\phi_i^2X_{n-2i} + 2\sum_{k=i}^{\lfloor\frac{p-1}{2}\rfloor}\phi_i\phi_{2k+1}X_{n-2k-2}\right).
\label{cast-final}
\end{equation}
%\begin{dmath}
%\sum_{i=1}^p(-1)^{i+1}\phi_i\sum_{k=1}^p\phi_kX_{n-k-i} = 
%	\phi_1^2X_{n-2}+2\phi_1\sum_{k=1}^{\left[\frac{p-1}{2}\right]}\phi_{2k+1}X_{n-2-2k} + \sum_{i=2}^p (-1)^{i+1}\phi_i\sum_{k=2}^p\phi_kX_{n-k-i} = 
%	\phi_1^2X_{n-2} +2\phi_1\sum_{k=0}^{\left[\frac{p-1}{2}\right]}\phi_{2k+1}X_{n-2-2k} - \phi_2^2X_{n-4} - 2\phi_2\sum_{k=0}^{\left[\frac{p-2}{2}\right]}\phi_{2k+2}X_{n-2k-4} - \sum_{i=2}^{p-1}(-1)^{i+1}\phi_{i+1}\sum_{k=2}^{p-1}\phi_{k+1}X_{n-i-k-2}=
%\sum_{i=1}^p(-1)^{i+1}\left(\phi_i^2X_{n-2i} + 2\sum_{k=0}^{\left[\frac{p-i}{2}\right]}\phi_{2k+i}X_{n-2(k+i)}\right).
%\label{eq:cast}
%\end{dmath}
%We intend that, when $i>\left\lfloor\frac{p-1}{2}\right\rfloor$, the last sum in Eq.~\eqref{cast-final} is zero. 
Eq.~\eqref{cast-final} shows that, after the decimation, one maintains an autoregressive part of order $p$. The picture is not modified by sum \encircle{A}, which is equal to 
\begin{equation}
{\encircle A}  = \sum_{i=1}^p(-1)^{i+1}\phi_i\sum_{k=1}^p\phi_kX_{n-k-i}+\mu_0\epsilon_n = 2\sum_{i=1}^{\lfloor p/2\rfloor}\phi_{2i}X_{n-2i}
\end{equation} 
and only contributes up to an AR order $\lfloor p/2\rfloor$. 

Thus Eq.~\eqref{cg-pq} can be rewritten as:
\begin{dmath}
X_n = \sum_{i=1}^{\lfloor p/2\rfloor}2\phi_{2i}X_{n-2i} + 
\sum_{i=1}^p(-1)^{i+1}\left(\phi_i^2X_{n-2i} + 2\sum_{k=i}^{\lfloor \frac{p-1}{2}\rfloor}\phi_i\phi_{2k+1} X_{n-2k-2}\right)+ \tilde r_n,
\label{cg-double}
\end{dmath}
where it is possible to recognize a structure of the following kind
\begin{equation}
X_n = \sum_{i=1}^p \tilde \phi_i X_{n-2i} + \tilde r_n.
\end{equation}
The process corresponds to an ARMA model with the same autoregressive order as the original one ($p$), but jumps cover time intervals of doubled amplitude. Further manipulation of the sums \encircle{A} and \encircle{B} in Eq.~\eqref{cg-pq} allows us to find formal expressions for the effective AR coefficients of the coarse grained process, $\tilde \phi_{i=1\dots p}$: 
\begin{equation}
\begin{cases}
\tilde \phi_1 = 2\phi_2 +\phi_1^2 ;\\
\tilde \phi_i = 2\phi_{2i} + (-1)^{i+1}\phi_i^2 + 2\phi_{2i-1}\sum_{k=1}^{i-1}(-1)^{k+1}\phi_k \quad \text{ for}\quad 2\leq i \leq \left\lfloor\frac{p}{2}\right\rfloor-1;\\
\tilde \phi_i = (-1)^{i+1}\phi_i^2 \hspace{5.45cm} \text{ for}\quad \left\lfloor\frac{p}{2}\right\rfloor+1 \leq i \leq p.
\end{cases}
\end{equation}
The coarse-grained coefficient $\tilde \phi_{\lfloor p /2 \rfloor}$ takes a different form depending on $p$ being even or odd:
\begin{flalign}
p \text{ odd}: \qquad \tilde \phi_{\lfloor p/2\rfloor} &= 2\phi_{2\lfloor p/2\rfloor} + (-1)^{1+\lfloor p/2\rfloor}\phi_{\lfloor p/2\rfloor}^2 ;\\
p \text{ even}: \qquad \tilde \phi_{\lfloor p/2\rfloor} &= 2\phi_{2\lfloor p/2\rfloor} + (-1)^{1+\lfloor p/2\rfloor}\phi_{\lfloor p/2\rfloor}^2 + 2\phi_{2\lfloor p/2\rfloor-1}\sum_{k=1}^{\left\lfloor \frac{p-1}{2}\right\rfloor}(-1)^{k+1}\phi_k.
\end{flalign}

What remains to determine is whether there is an invariant MA order $q$ associated to $p$. Let us restart from Eq.\eqref{cg-pq} and focus on the random term:
\begin{equation}
\tilde r_n = \mu_0\epsilon_n + \sum_{j=1}^q\mu_j\epsilon_{n-j} + \sum_{i=1}^p (-1)^{i+1}\phi_i\left(\mu_0\epsilon_{n-i}+\sum_{j=1}^q\mu_j\epsilon_{n-j-i}\right).
\end{equation}
Since linear combinations of Gaussian variables are still Gaussian, one can properly redefine the $\epsilon_m$'s and rearrange the coefficients in front of them to rewrite $\tilde r_n=\sum_{i=0}^{\tilde q}\tilde\mu_i\epsilon_{n-2i}$, where 
\begin{equation}
\tilde q=\left\lfloor \frac{p+q}{2}\right\rfloor.
\end{equation}

Hence one can deduce that there are only 2 invariant scenarios for ARMA($p,q$) processes: $q=p$ or $q=p-1$. When translated into the language of integration schemes for continuous-time processes, this fact tells us that partial observation let memory emerge: each hidden degree of freedom increases by one the order of both the AR part and the MA part of the discrete model, thus introducing color, as expected \cite{Zwanzig-book, Horenko}.

Once the general invariant structure under decimation of ARMA($p,q$) time series is found, the RG machinery can be deployed, and a careful study of the fixed points can be carried out. In order to complete the RG step and obtain explicit flow equations, it is necessary to detail the rescaling operation.
To this purpose, it is convenient to expand any coefficient of the ARMA($p,q$) model as a power series of the time step $\tau$. If we interpret the ARMA model as a discretization of a continuous time process, the discrete model parameters are indeed dimensionless functions of $\tau$, and it is not clear how they should be rescaled. In order to fix this problem, we resort to an asymptotic expansion in power series: to work exclusively with integer powers of $\tau$, we replace the set of parameters $\{\phi_{i=1\dots p},\nu_{i=1\dots q},\mu\}$ with the equivalent set $\{\phi_{i=1\dots p},\gamma_{k=1\dots q+1}\}$, where 
\begin{equation}
\gamma_k = \Exp{r_nr_{n+k}}.
\label{gamma-def}
\end{equation}
Any parameter $A$ in the new set can be expressed as $A = \sum_{k=0}^{\infty} A_k \tau^k$. The infinite collection of coefficients $A_k$ constitute the parameter space of our model. Upon rescaling of the time unit, each of them is now rescaled, after coarse-graining, according to its physical dimension: $2^{-k}\tilde A_k$, with $\tilde A_k$ the coarse-grained parameter. This completes the prescription to derive the RG map for the considered class of linear time series models.

\begin{figure}[t]
\centering
\includegraphics[width=.45\columnwidth]{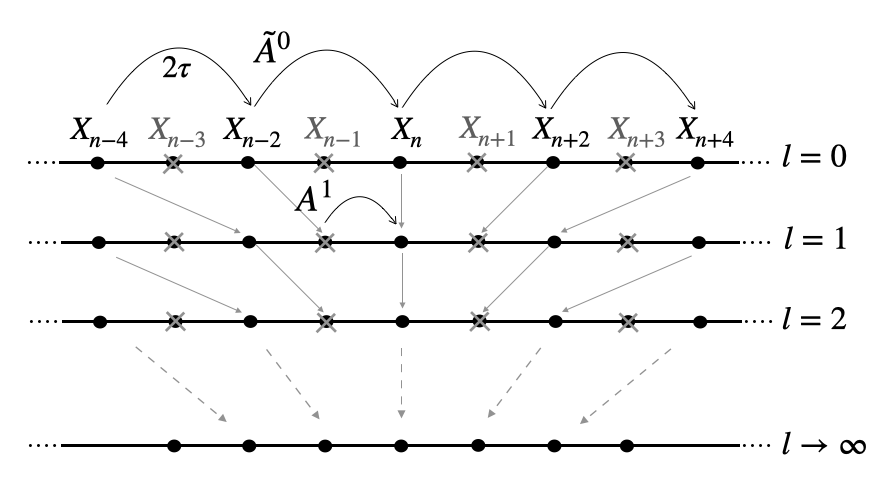}\llap{
  \parbox[b]{1.2cm}{a\\\rule{0ex}{1.5in}}}%\llap{
 % \parbox[b]{5cm}{\tiny{\textbf{RG SCHEME}}\\\rule{0ex}{1.05in}}}\llap{
 % \parbox[b]{10.1cm}{\tiny{$l=0$}\\\rule{0ex}{.98in}}}\llap{
 % \parbox[b]{10.1cm}{\tiny{$l=1$}\\\rule{0ex}{.78in}}}\llap{
 % \parbox[b]{10.1cm}{\tiny{$l=2$}\\\rule{0ex}{.58in}}}\llap{
 % \parbox[b]{9.9cm}{\tiny{$l\to \infty$}\\\rule{0ex}{.27in}}}
 \hfill
\includegraphics[width=.45\columnwidth]{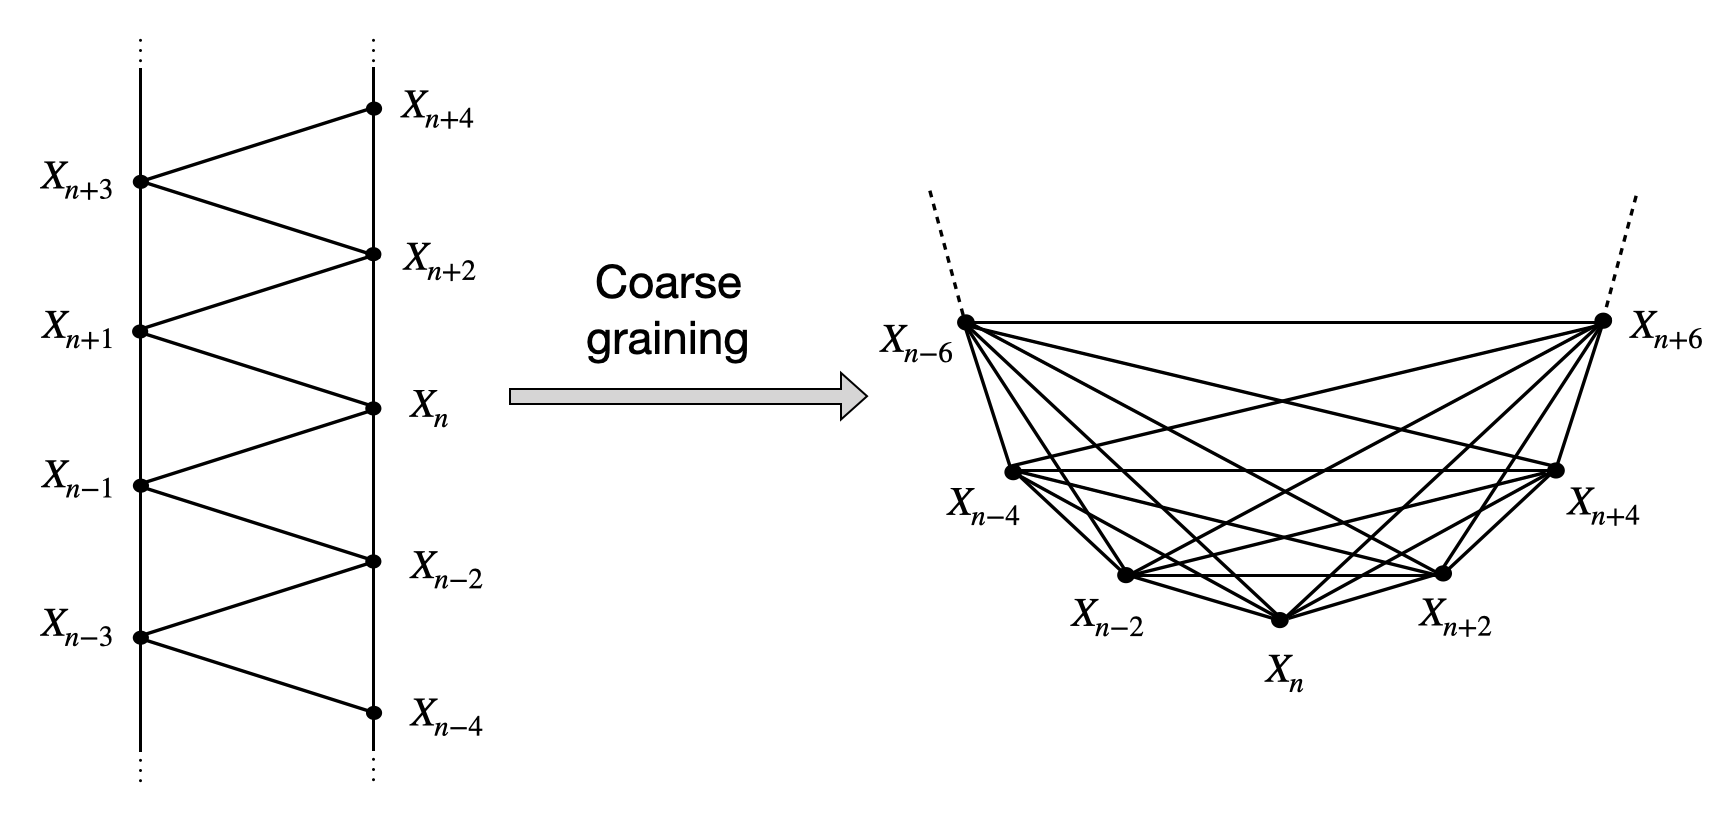}\llap{
  \parbox[b]{1.2cm}{b\\\rule{0ex}{1.3in}}}
\caption{(a) Sketch of the RG procedure for ARMA processes: the discrete times series is firstly decimated and then rescaled, so that the time step/lattice spacing is always kept equal to $\tau$. Cfr. Fig.1 in the main text. (b) In the case of second order processes, the Euler starting point ---AR(2) time series--- corresponds to a spin chain model with nearest-neighbor and next-nearest-neighbor couplings, which can also be represented as a zig-zag ladder. The ladder structure is not invariant under real space RG transformations. The decimation procedure sketched in (a) produces, since the first iteration, infinite range couplings. However, these couplings are not independent, and the 4 parameters of the ARMA(2,1) model $\phi_1=\psi$, $\phi_2=\theta$, $\mu$ and $\nu_1=\nu$ are sufficient to characterize them.}
\label{fig:schematic}
\end{figure}

%%%%%%%%%%%%%%%%%%%%%%%%%%%%%%%%%%%%%%%%%%%%%%%%%%%%%%%%%%%%%%
%%%%%%%%%%%%%%%%%%%%%%%%%%%%%%%%%%%%%%%%%%%%%%%%%%%%%%%%%%%%%%
\section*{II. Renormalization Group for ARMA(2,1) processes}

In the following, we will focus on the case of ARMA(2,1) processes.
The starting point of interest for us is indeed the Euler discretization of the following additive linear process (i.e. the stochastic harmonic oscillator):
\begin{flalign}
	\label{xgen}dx &= vdt\\
	\label{vgen}dv &= -\eta vdt - \kappa x dt +\sigma dW,
\end{flalign}
which corresponds to the AR(2) process
\begin{equation}
	X_{n+1} - 2X_n + X_{n-1} + \eta\tau (X_n - X_{n-1}) + \kappa\tau^2 X_{n-1} = \sigma\tau^{3/2}\epsilon_{n+1}.
	\label{Euler-ho}
\end{equation}
As before, $\epsilon_n\sim\mathcal N(0,1)$ I.I.D.. We can also rename $\psi = 2-\eta\tau$ ($\phi_1$ in the notation above), $\theta = -1+\eta\tau-\kappa\tau^2$ ($\phi_2$ in the notation above), $\mu=\sigma\tau^{3/2}$, so that Eq.~\eqref{Euler-ho} is rewritten as: 
\begin{equation}
	X_n = \psi X_{n-1} + \theta X_{n-2} + \mu \epsilon_n. 
	\label{eq:AR2}
\end{equation}
Coarse graining is obtained for any ARMA(2,$q$) process by taking the combination $\text{Eqn}(X_n) + \psi \text{Eqn}(X_{n-1}) - \theta \text{Eqn}(X_{n-2})$ (see Sec.~\ref{sec:arma-gen} and recall $\psi = \phi_1$, $\theta=\phi_2$). Explicitly, it reads:
\begin{equation}
X_n + \psi X_{n-1} - \theta X_{n-2} = \psi X_{n-1} + \theta X_{n-2} + \mu \epsilon_n+ \psi \left( \psi X_{n-2} + \theta X_{n-3} + \mu \epsilon_{n-1}\right)-\theta \left( \psi X_{n-3} + \theta X_{n-4} + \mu \epsilon_{n-2}\right),
\end{equation}
and yields a dynamical law for the `even sub-series' of states of the following kind:
\begin{equation}
	X_n = \tilde \psi X_{n-2} + \tilde \theta X_{n-4} +\tilde r_n,
\end{equation}
where $\tilde r_n$ is the random increment of the coarse-grained process. If we start from the AR(2) process \eqref{eq:AR2}, i.e. $q=0$, the new parameters are $\tilde \psi = (\psi^2+2\theta)$, $\tilde\theta = -\theta^2$, and the new random increment $\tilde r_n$ is defined as 
\begin{equation}
\tilde r_n = \mu\left[\epsilon_n +\psi\epsilon_{n-1}-\theta\epsilon_{n-2}\right].
\end{equation}
Thus, $\Exp {\tilde r_n \tilde r_{n\pm2}}\neq 0$, meaning that at the first iteration we already fall in the class of ARMA(2,1) models. Luckily, the ARMA(2,1) structure is left unchanged by further iterations of this procedure, as shown in Sec~\ref{sec:arma-gen}. 

Therefore, let us focus on the ARMA(2,1) model. The starting point at the $l$-th iteration is given by:
\begin{equation}
	X_n = \psi^{l} X_{n-1} + \theta^{l} X_{n-2} +\mu^{l}\epsilon_n + \nu^{l}\epsilon_{n-1}
\end{equation}
with running parameters $\psi^{l}$, $\theta^{l}$, $\mu^{l}$, $\nu^{l}$. Applying the aforementioned combination gives the coarse-grained stochastic difference equation
\begin{equation}
	X_n = \left((\psi^{l})^2+2\theta^{l}\right)X_{n-2} - (\theta^{l})^2X_{n-4} + \tilde r_n^{l}
\end{equation}
where 
\begin{equation}
\tilde r_n^{l}=\mu^{l}\epsilon_n +(\nu^{l}+\psi\mu^{l})\epsilon_{n-1} + (\psi\nu^{l}-\theta\mu^{l})\epsilon_{n-2} - \theta\nu^{l}\epsilon_{n-3}.
\end{equation}
Thus the covariance of the series of random increments is specified by
\begin{flalign}
\label{rec-mu}&\Exp{ (\tilde r_n^{l})^2} = \left[(\mu^{l})^2+(\nu^{l})^2\right]\left[1+(\psi^{l})^2+(\theta^{l})^2\right] + 2\mu^{l}\nu^{l}\psi^{l}\left(1-\theta^{l}\right);\\%\coloneqq \tilde\alpha^{(l)}\sigma^2;
\label{rec-nu}&\Exp{ \tilde r_n^{l} \tilde r_{n\pm2}^{l}} = \mu^{l}\nu^{l}\psi^{l}\left(1-\theta^{l}\right)-\theta^{l}\left[(\mu^{l})^2+(\nu^{l})^2\right].%\coloneqq \tilde\beta^{(l)}\sigma^2.
\end{flalign}
For a linear additive process like the one we considered above, the covariance matrix is a symmetric tridiagonal Toeplitz matrix, fully characterized by these two entries. It can be easily verified that $\Exp{\tilde r_n^l \tilde r_{n\pm2k}^l}=0$ for $k>1$. 

At this point, one can exploit the fact that linear combinations of Gaussian variables are Gaussian. Hence the random increment $\tilde r_n^{l}$ is decomposed in the following way:
\begin{equation}
	\tilde r_n^{l} = \tilde\mu^{l}\tilde\epsilon_n + \tilde\nu^{l}\tilde\epsilon_{n-2},
\end{equation}
with $\tilde\epsilon_i\sim\mathcal N(0,1)$ new I.I.D. variables, and $\tilde\mu^{l}$, $\tilde\nu^{l}$ satisfying:
\begin{equation}
	\Exp{ (\tilde r_n^{l})^2}= (\tilde\mu^{l})^2 + (\tilde\nu^{l})^2;\qquad
	\Exp{ \tilde r_n^{l} \tilde r_{n\pm2}^{l}} = \tilde\mu^{l} \tilde\nu^{l}. %= \mu^{l}\nu^{l}\phi_1^{l}(1-\phi_2^{l})-\phi_2^{l}\left[(\mu^{l})^2 +(\nu^{l})^2\right].
	\label{mu-nu-def}
\end{equation}
Let us introduce the two running parameters $\alpha^l={(\mu^l)}^2 +{(\nu^l)}^2$ and $\beta^l=\mu^l\nu^l$ -- corresponding to $\gamma_0$ and $\gamma_1$ of Eq.~\eqref{gamma-def} -- such that Eqs.~\eqref{rec-mu} and \eqref{rec-nu}, combined with Eq.~\eqref{mu-nu-def}, become:
\begin{flalign}
	\label{tilde-a}&\tilde\alpha^{l} = \left[1+(\psi^{l})^2 +(\theta^{l})^2\right]\alpha^{l} + 2\psi^{l}(1-\theta^{l})\beta^{l};\\
	\label{tilde-b}&\tilde\beta^{l} = \psi^{l}(1-\theta^{l})\beta^{l} - \theta^{l}\alpha^{l}.
\end{flalign}

Let us now consider a power series expansion for all the parameters at stake:
\begin{flalign}
%\label{coef-1}\phi_1 = \psi_0 + \psi_1\tau + \psi_2\tau^2 + \psi_3\tau^3 + o(\tau^3);\quad \phi_2 = \theta_0 + \theta_1\tau + \theta_2\tau^2 + \theta_3\tau^3 + o(\tau^2); \\
\label{coef-1}\psi^{l} =\sum_{k=0}^{\infty} \psi_k^{l}\tau^k;\quad \theta^{l} =\sum_{k=0}^{\infty} \theta_k^{l}\tau^k\\
%\label{coef-2}\alpha = \alpha_0 + \alpha_1\tau + \alpha_2\tau^2 + \alpha_3\tau^3 + o(\tau^3);\quad \beta = \beta_0 + \beta_1\tau + \beta_2\tau^2 + \beta_3\tau^3 + o(\tau^3).
\label{coef-2}\alpha^{l} = \sum_{k=0}^{\infty} \alpha_k^{l}\tau^k;\quad \beta^{l} = \sum_{k=0}^{\infty}\beta_k^{l}\tau^k.
\end{flalign}
This expansion is necessary because the parameters of the ARMA(2,1) model are dimensionless, and it would not be clear how to perform the rescaling step on them otherwise.
Each coefficient in the series expansions~\eqref{coef-1}--\eqref{coef-2} has a well-defined physical dimension (in time units), and must be interpreted as a running parameter that gets rescaled according to it:
\begin{equation}
A_k^{l+1} = 2^{-k} \tilde A_k^{l}
\label{rescA}
\end{equation}
Recurrence equations are then obtained applying \eqref{rescA}
to Eqs.~\eqref{tilde-a}--\eqref{tilde-b} and to the coarse-grained AR coefficients:
\begin{equation}
\tilde \psi^{l} = (\psi^{l})^2 + 2\theta^{l};\qquad \tilde\theta^{l} = -(\theta^{l})^2.
\label{tilde-phi}
\end{equation}
Equating order by order, one finally finds a layered set of recurrence relations that we analyze in the following sections.

\subsection{AR coefficients}
Since the recurrence relations for $\psi$ and $\theta$ are independent of those for $\alpha$ and $\beta$, let us start with the coefficients of the autoregressive (AR) part of the model. Using Eqs.~\eqref{coef-1} and ~\eqref{tilde-phi} one finds
\begin{equation}
 \tilde\psi_k^{l} = 2\theta_k^l + \sum_{i=0}^k\psi_i^l\psi_{k-i}^l;\qquad
 \tilde\theta_k^{l} = - \sum_{i=0}^k\theta_i^l\theta_{k-i}^l.
 \label{general-AR}
\end{equation}
Recalling from Eq.~\eqref{rescA} that $\psi_k^{l+1}=2^{-k}\tilde \psi^{l}_k$ and  $\theta_k^{l+1}=2^{-k}\tilde \theta^{l}_k$, recursive relations are readily obtained. 
At each order $k$ of the series expansion we obtain a two-dimensional map from which the fixed points for the considered coefficients, $(\psi_k^*,\theta_k^*)$, can be extracted. Notice that higher order recurrence relations are coupled to lower order ones, so one can follow a typical multiscale approach to find the fixed points or solve the recurrence relations. Here we are just interested in the study of the fixed points.


\subsubsection*{0-th order}
The recursive relations at the leading order read:
\begin{equation}
\begin{cases}
\psi_0^{l+1} = (\psi_0^{l})^2 + 2\theta_0^{l}\\
\theta_0^{l+1} = -(\theta_0^{l})^2.
\end{cases}
\label{map0}
\end{equation}
As it is evident from Eq.~\eqref{general-AR}, only at this order the system is nonlinear; at any subsequent order the map is linear. There are 4 fixed points for the nonlinear recurrence relation Eq.~\eqref{map0}:
\begin{enumerate}
\item[A.] $(\psi_0^*,\theta_0^*) = (0,0)$. This is a process with null autoregressive part, i.e. a pure moving average (MA) process. %Moving average contributions (eventually null) are specified by the recurrence relations for the MA coefficients. 
\item[B.] $(\psi_0^*,\theta_0^*) = (1,0)$.  This fixed point corresponds to a first order process of the form $X_n  = X_{n-1} + r_n$, i.e. an ARMA(1,$q$) process; the moving average order $q$ will be determined by the recurrence relations for $\alpha_k$ and $\beta_k$.
\item[C.] $(\psi_0^*,\theta_0^*) = (-1,-1)$. This is an ARMA(2,$q$) process, of the form $X_n = -X_{n-1}-X_{n-2}+r_n$. Here again, the random contribution will be specified by the recursion relations for $\alpha_k$ and $\beta_k$. %\textcolor{red}{I think it's also an unstable process, in typical ARMA meaning}
\item[D.] $(\psi_0^*,\theta_0^*) = (2,-1)$. This model is a specific case of an ARMA(2,$q$) model, known as ARIMA(1,1,$q$) model \cite{Brockwell-Davis-book}. Thanks to the specific value assumed by the coefficients of the AR part, one can indeed rewrite the process as $(1-L)^2X_{n} = r_n$, where $L$ is the lag operator: $LX_n = X_{n-1}$. So $(1-L)$ is the discrete differencing operator and $\{(1-L)X_n\}=\{\bar V_n\}$ is the reconstructed velocity series. We leave once again the value of $q$ unspecified for the moment, as it is determined by the analysis of the recurrence relations for the MA coefficients.
\end{enumerate}
Notice that only the fixed point A is an asymptotically stable point, whose basin of attraction is the interior of the triangle in Fig.~\ref{fig:rec_rel}a. The other points are unstable, at least in some directions. 

We are especially interested in the class of discrete-time models represented by point D, since, at the leading order, the model can be considered as a discretized version of a second order SDE of the kind $\ddot x = \xi$, with $\xi(t)$ a white or colored Gaussian noise. Higher order contributions can modify the coefficients $\phi_1=\psi$ and $\phi_2=\theta$ in front of $X_{n-1}$ and $X_{n-2}$, but they won't affect the interpretation of such a process as a discretization of a second order SDE; the only difference will be in the addition of position- or velocity-dependent linear forces.

\subsubsection*{1st order}
The recurrence relations for first-order coefficients read:
\begin{equation}
\begin{cases}
\psi_1^{l+1} = \frac{1}{2}\left[2\psi_0^{l}\psi_1^{l} + 2 \theta_1^{l}\right]\\
\theta_1^{l} = \frac{1}{2}\left[-2\theta_0^{l}\theta_1^{l}\right].
\end{cases}
\end{equation}
The study of the fixed points reveals that their number and their nature (i.e. the kind of dynamical models they correspond to) is left unchanged:
\begin{enumerate}
\item[A.] $(\psi_0^*,\theta_0^*)=(0,0) \implies (\psi_1^*,\theta_1^*) =(0,0)$. The process is still a MA process.
\item[B.] $(\psi_0^*,\theta_0^*)=(1,0) \implies (\psi_1^*,\theta_1^*) =(u,0)$ where $u$ is a free parameter. The process is still an ARMA(1,$q$) process, but it is represented by a manifold of fixed points in the space of first order coefficients.
\item[C.] $(\psi_0^*,\theta_0^*)=(-1,-1) \implies (\psi_1^,\theta_1^*)=(u,2u)$. As for the previous fixed point, even for this unstable ARMA(2,$q$) process the dimension of the fixed point manifold is increased of one when we move from the 0-th order to the first order expansion.
\item[D.] $(\psi_0^*,\theta_0^*)=(2,-1) \implies (\psi_1^*,\theta_1^*)=(u,-u)$. In this case the equation of motion becomes $(1-L)(1-\psi_1^*L)X_n = r_n$, still corresponding to a class of ARIMA(1,1,$q$) processes.%, with $q\leq1$. 
\end{enumerate}

\subsubsection*{2nd order}
Given the recurrence relations:
\begin{equation}
\begin{cases}
\psi_2^{l+1} = \frac{1}{4}\left[2\psi_0^{l}\psi_2^{l} + (\psi_1^{l})^2 + 2\theta_2^{l}\right]\\
\theta_2^{l+1} = -\frac{1}{4}\left[2\theta_0^{l}\theta_2^{l}+(\theta_1^{l})^2\right],
\end{cases}
\end{equation}
the fixed points, at this order, are expanded as follows:
\begin{enumerate}
\item[A.] $(\psi_0^*,\theta_0^*,\psi_1^*, \theta_1^*)=(0,0,0,0) \implies (\psi_2^*,\theta_2^*)=(0,0).$ No increase in the dimension of the manifold nor change in the nature of the process is registered.
\item[B.] $(\psi_0^*,\theta_0^*,\psi_1^*,\theta_1^*)=(1,0,u,0) \implies (\psi_2^*,\theta_2^*) = (u^2/2,0)$. The ARMA(1,$q$) nature of the model is left unchanged.
\item[C.] $(\psi_0^*,\theta_0^*,\psi_1^*,\theta_1^*)=(-1,-1,u,2u) \implies (\psi_2^* ,\theta_2^*)=(-u^2/2,-2u^2)$. The values of these parameters are fixed by the values of lower order parameters, as it happened for the previous fixed point. Hence the dimension of the fixed point manifold does not change here, moving from first to second order expansion. 
\item[D.] $(\psi_0^*,\theta_0^*,\psi_1^*,\theta_1^*)=(2,-1,u,-u) \implies (\psi_2^*,\theta_2^*) = (z,-u^2/2)$. The additional arbitrariness on $\psi_2^*$ accommodates an $x$-dependent force in the second-order continuous-time SDE, from which the discrete model can be derived. The discretization picture above keeps holding, even if the ARIMA(1,1,$q$) structure is lost in favor of an ARMA(2,$q$) one, when $\psi_2^*\neq u^2/2$.
\end{enumerate}

\begin{figure}[t]
\centering
\includegraphics[width=.45\columnwidth]{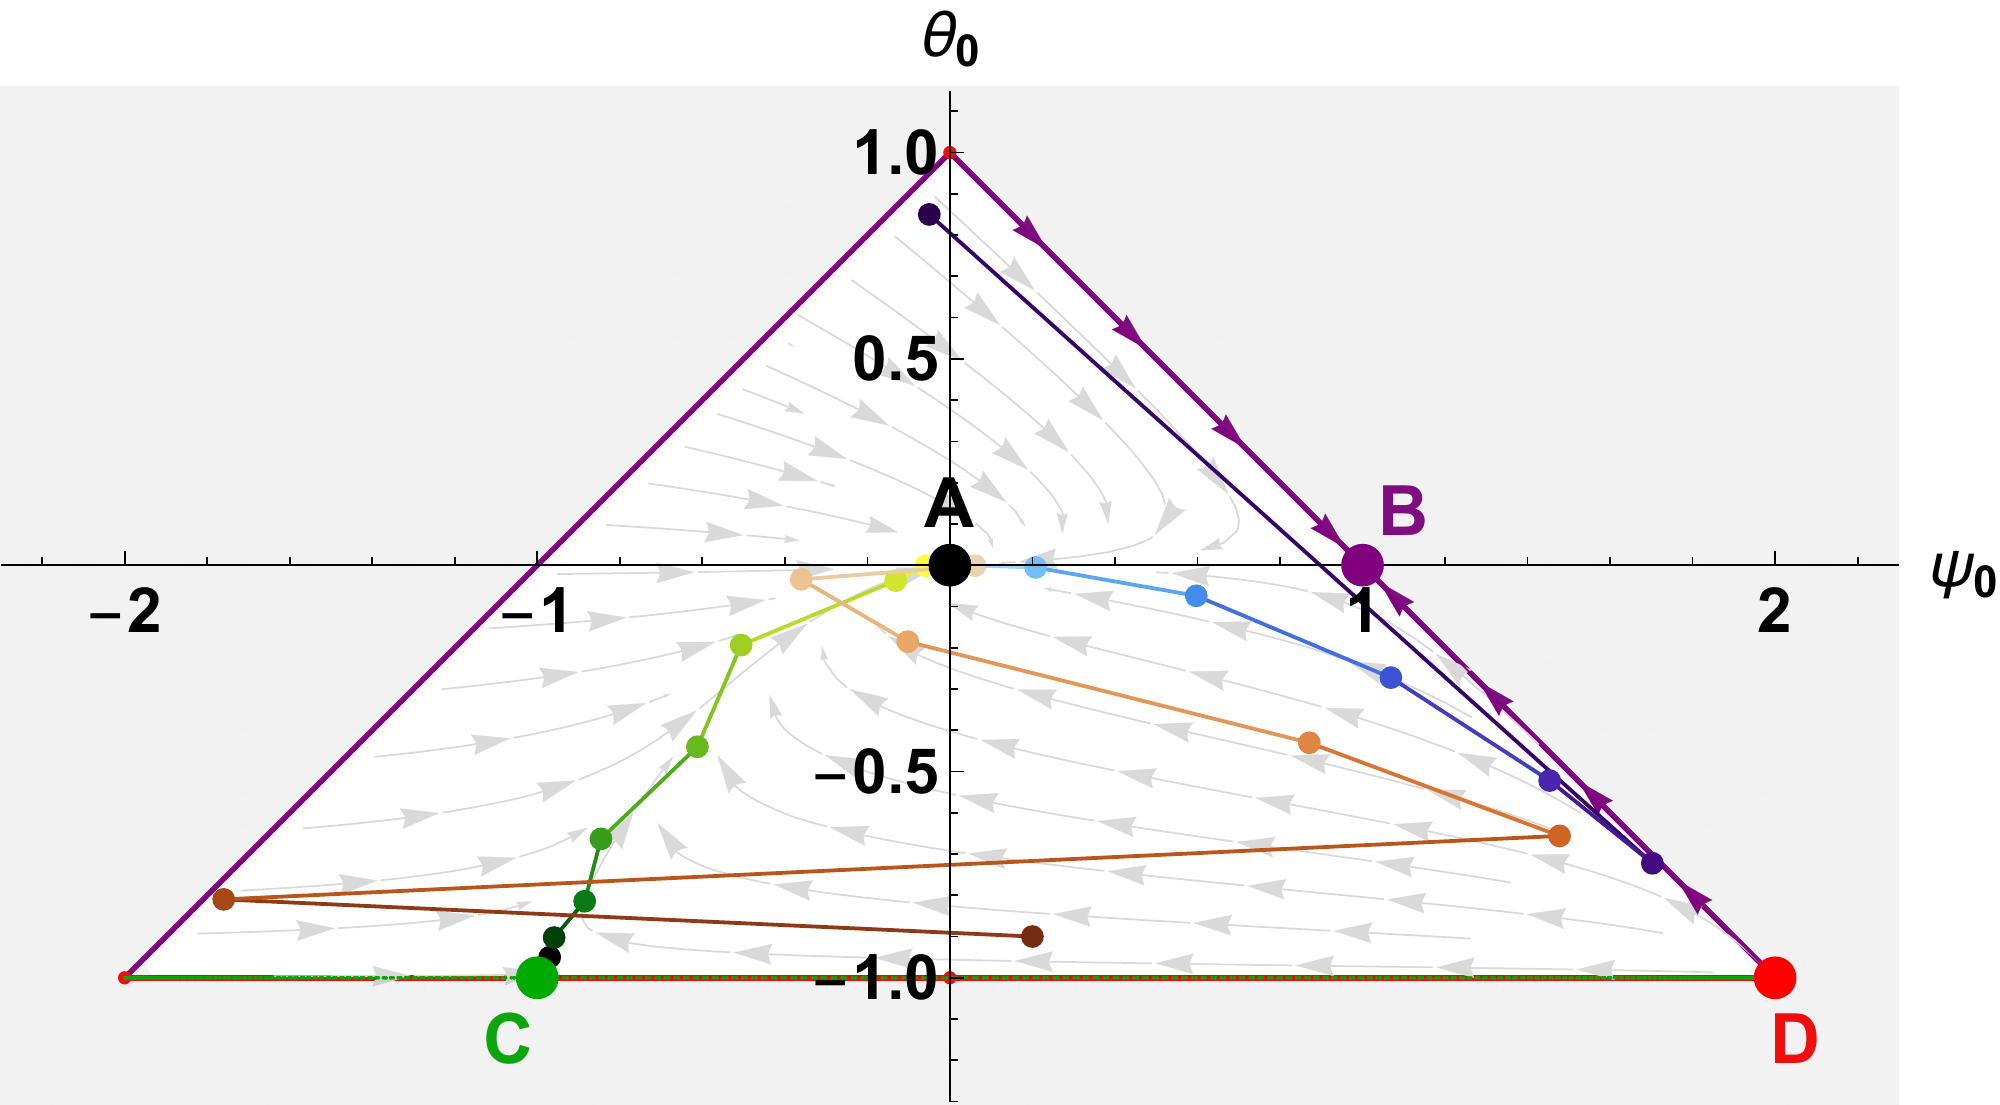}\llap{
  \parbox[b]{1.2cm}{a\\\rule{0ex}{1.5in}}}\hfill
\includegraphics[width=.45\columnwidth]{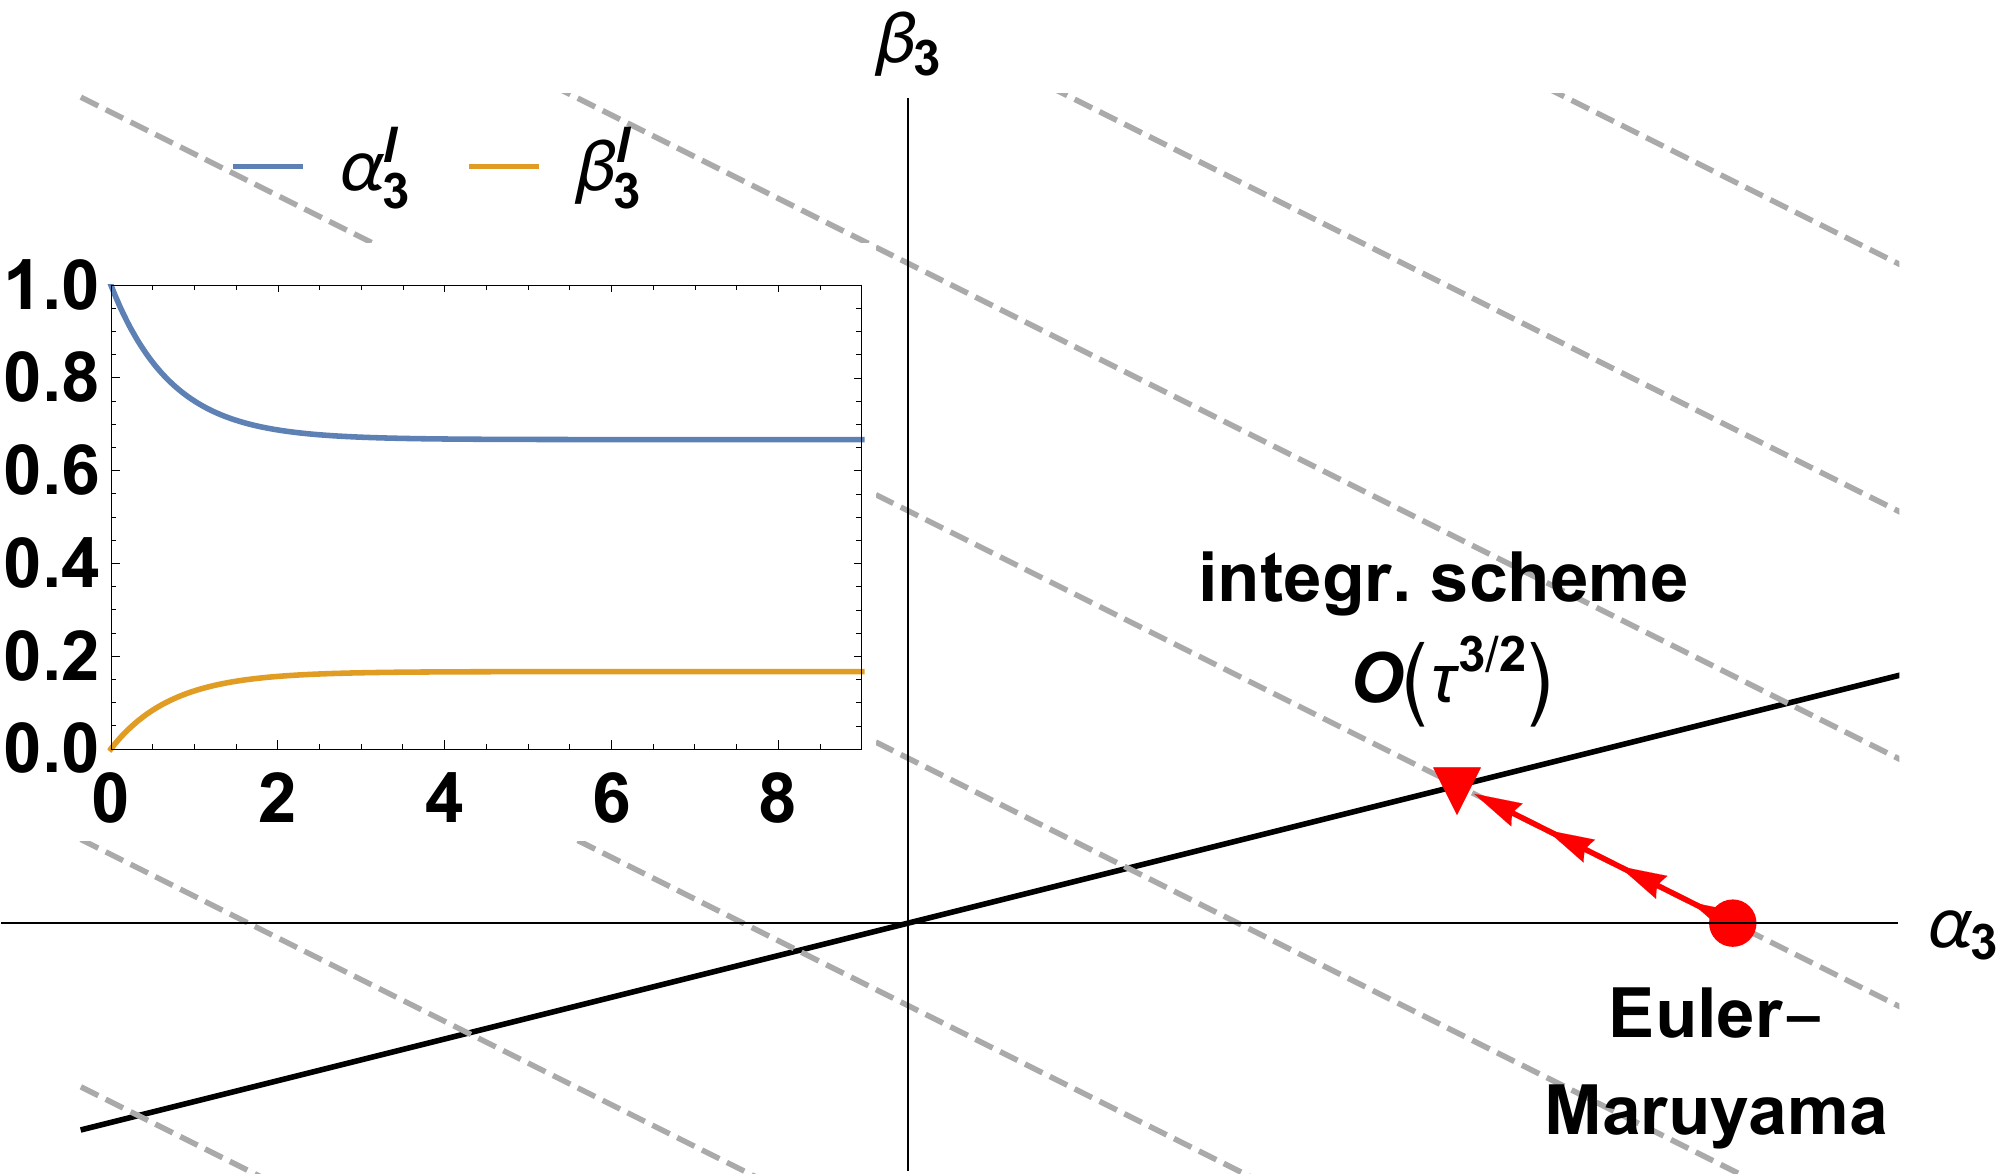}\llap{
  \parbox[b]{1.2cm}{b\\\rule{0ex}{1.5in}}}
\caption{(a) Fixed points on the plane of leading order AR coefficients. For a description of the figure, see the main text. (b) RG flow on the plane of third order MA coefficients for $s=0$. The black solid line is the manifold of fixed points $\alpha_3^* = 4 \beta_3^*$. The dashed parallel lines represent different orbits associated to the solution \eqref{sol-ab-3} of the linear system. A Euler-Maruyama discretization of a 2nd-order SDE corresponds to an initial condition $(\sigma^2,0)$ on the positive $\alpha_3$ axis, which flows towards the ARMA(2,1) fixed point of coordinates $(2/3,1/6)\sigma^2$ with an $l$-dependent decay shown in the inset. When $s\neq 0$ the picture above is just slightly modified, as the RG map becomes an affine one.}
\label{fig:rec_rel}
\end{figure}

\begin{table}[h] %add [H] placement to break table across pages
\caption{\label{tab:AR} 
Fixed points. The last model is, up to $O(\tau)$, an ARIMA(1,1,1), for any value of the free parameter $u$. 
}
\begin{ruledtabular}
\begin{tabular}{c c c  c c  c c  c c c}
\centering
& Model & $\psi_0^*$ & $\theta_0^*$ & $\psi_1^*$ & $\theta_1^*$ & $\psi_2^*$ & $\theta_2^*$ & $\psi_3^*$ & $\theta_3^*$ \\

A. & MA($q$) & 0 & 0 & 0 & 0 & 0 & 0 & 0 & 0\\
B. & ARMA(1,$q$) & 1 & 0 & $u$ & 0 & $u^2/2$ & 0 & $u^3/6$ & 0 \\
C. &  ARMA(2,$q$) & -1 & -1 & $u$ & $2u$ & $-u^2/2$ & $-2u^2$ & $u^3/6$ & $(2u)^3/6$\\
D. &  AR(I)MA(2,$q$) & 2 & -1 & $u$ & $-u$ & $z$ & $-u^2/2$ & $u(6z-u^2)/12$ & $-u^3/6$\\
\end{tabular}
\end{ruledtabular}
\end{table}


Of course the study of the fixed points can be developed to any desired order, but the discussion we made so far is already sufficient to characterize their autoregressive nature. We summarize in Table \ref{tab:AR} the results for the AR coefficients of the series expansion up to the third order. %Going at least to the third order is necessary for the following discussion about MA coefficients. 
The fact that the AR order of the fixed points is left unchanged at subsequent orders in the expansion can be proven by induction on Eq.~\eqref{general-AR}. Specifically, the following facts hold:
\begin{enumerate}
\item The autoregressive (AR) order of fixed point A is exactly zero, since $\psi_k=\theta_k=0$ $\forall k$.
\item For fixed point B, $\theta_k=0$ $\forall k$, ensuring it is a process of AR order equal to one. Since $\psi_k = \frac{\psi_1^k}{k!}$, the non-vanishing autoregressive parameter is $\psi(\tau) = e^{\psi_1\tau}$. This fixed point corresponds to the exact discretization of a first order linear process, whose deterministic part reads $\dot x = \psi_1 x$, with $\psi_1=u$ arbitrary parameter.
\item Fixed point C satisfies $\psi_k = -\frac{(-\psi_1)^k}{k!}$ and $\theta_k = -\frac{(-2\psi_1)^k}{k!}$, implying $\psi(\tau)=-e^{-\psi_1\tau}$ and $\theta(\tau)=-e^{-2\psi_1\tau}$. As far as we know, this class model does not play any central role in physical processes. The process has a three-branched phase diagram, and evolves in time jumping from one branch to the next one -- approaching the origin or moving away from it depending on the sign of $\psi_1$ (see Fig.~\ref{fig:non-phys}). This structure is invariant under the RG transformation we defined, but it is precisely determined by the details of the decimation procedure. If the coarse graining procedure was implemented differently, for instance by trimming two points out of three, the same type of process would not be a fixed point. Trimming two points out of three in Fig.~\ref{fig:non-phys} would result into a single-branched phase diagram.
\item For fixed point D we have $\theta_k=-\frac{\psi_1^k}{k!}$, so that $\theta(\tau) = -e^{\psi_1\tau}$. As regards the other AR parameter, one can prove by induction that $\psi_0=2$, $\psi_{k\geq1}=\frac{\psi_1^k}{k!}$ is a fixed point solution, corresponding to $\psi(\tau)=1+e^{\psi_1\tau}$. The associated $z$ parameter is equal to $\psi_1^2/2$ in Table \ref{tab:AR}. In this case the process is an ARIMA(1,1,$q$) model, the deterministic part being the discretization of a linear first order process for the velocity variables $v=\dot x$: $\ddot x = \psi_1\dot x$. This is not, however, the only fixed point solution; additional arbitrariness, expressed by the free parameter $z$, can be accommodated to take into account additional elastic forces (see Sec.~\ref{sec:4fp}). %, which transform the previous equation into $\ddot x = \psi_1 \dot x - \kappa x$, where the $\kappa$ parameter is a function of $\psi_1$ and $\psi_2$. %We don't have a simple formula for $\psi_k$ that is valid at any $k$ in this case.
\end{enumerate}

\begin{figure}
\centering
\includegraphics[width=.32\columnwidth]{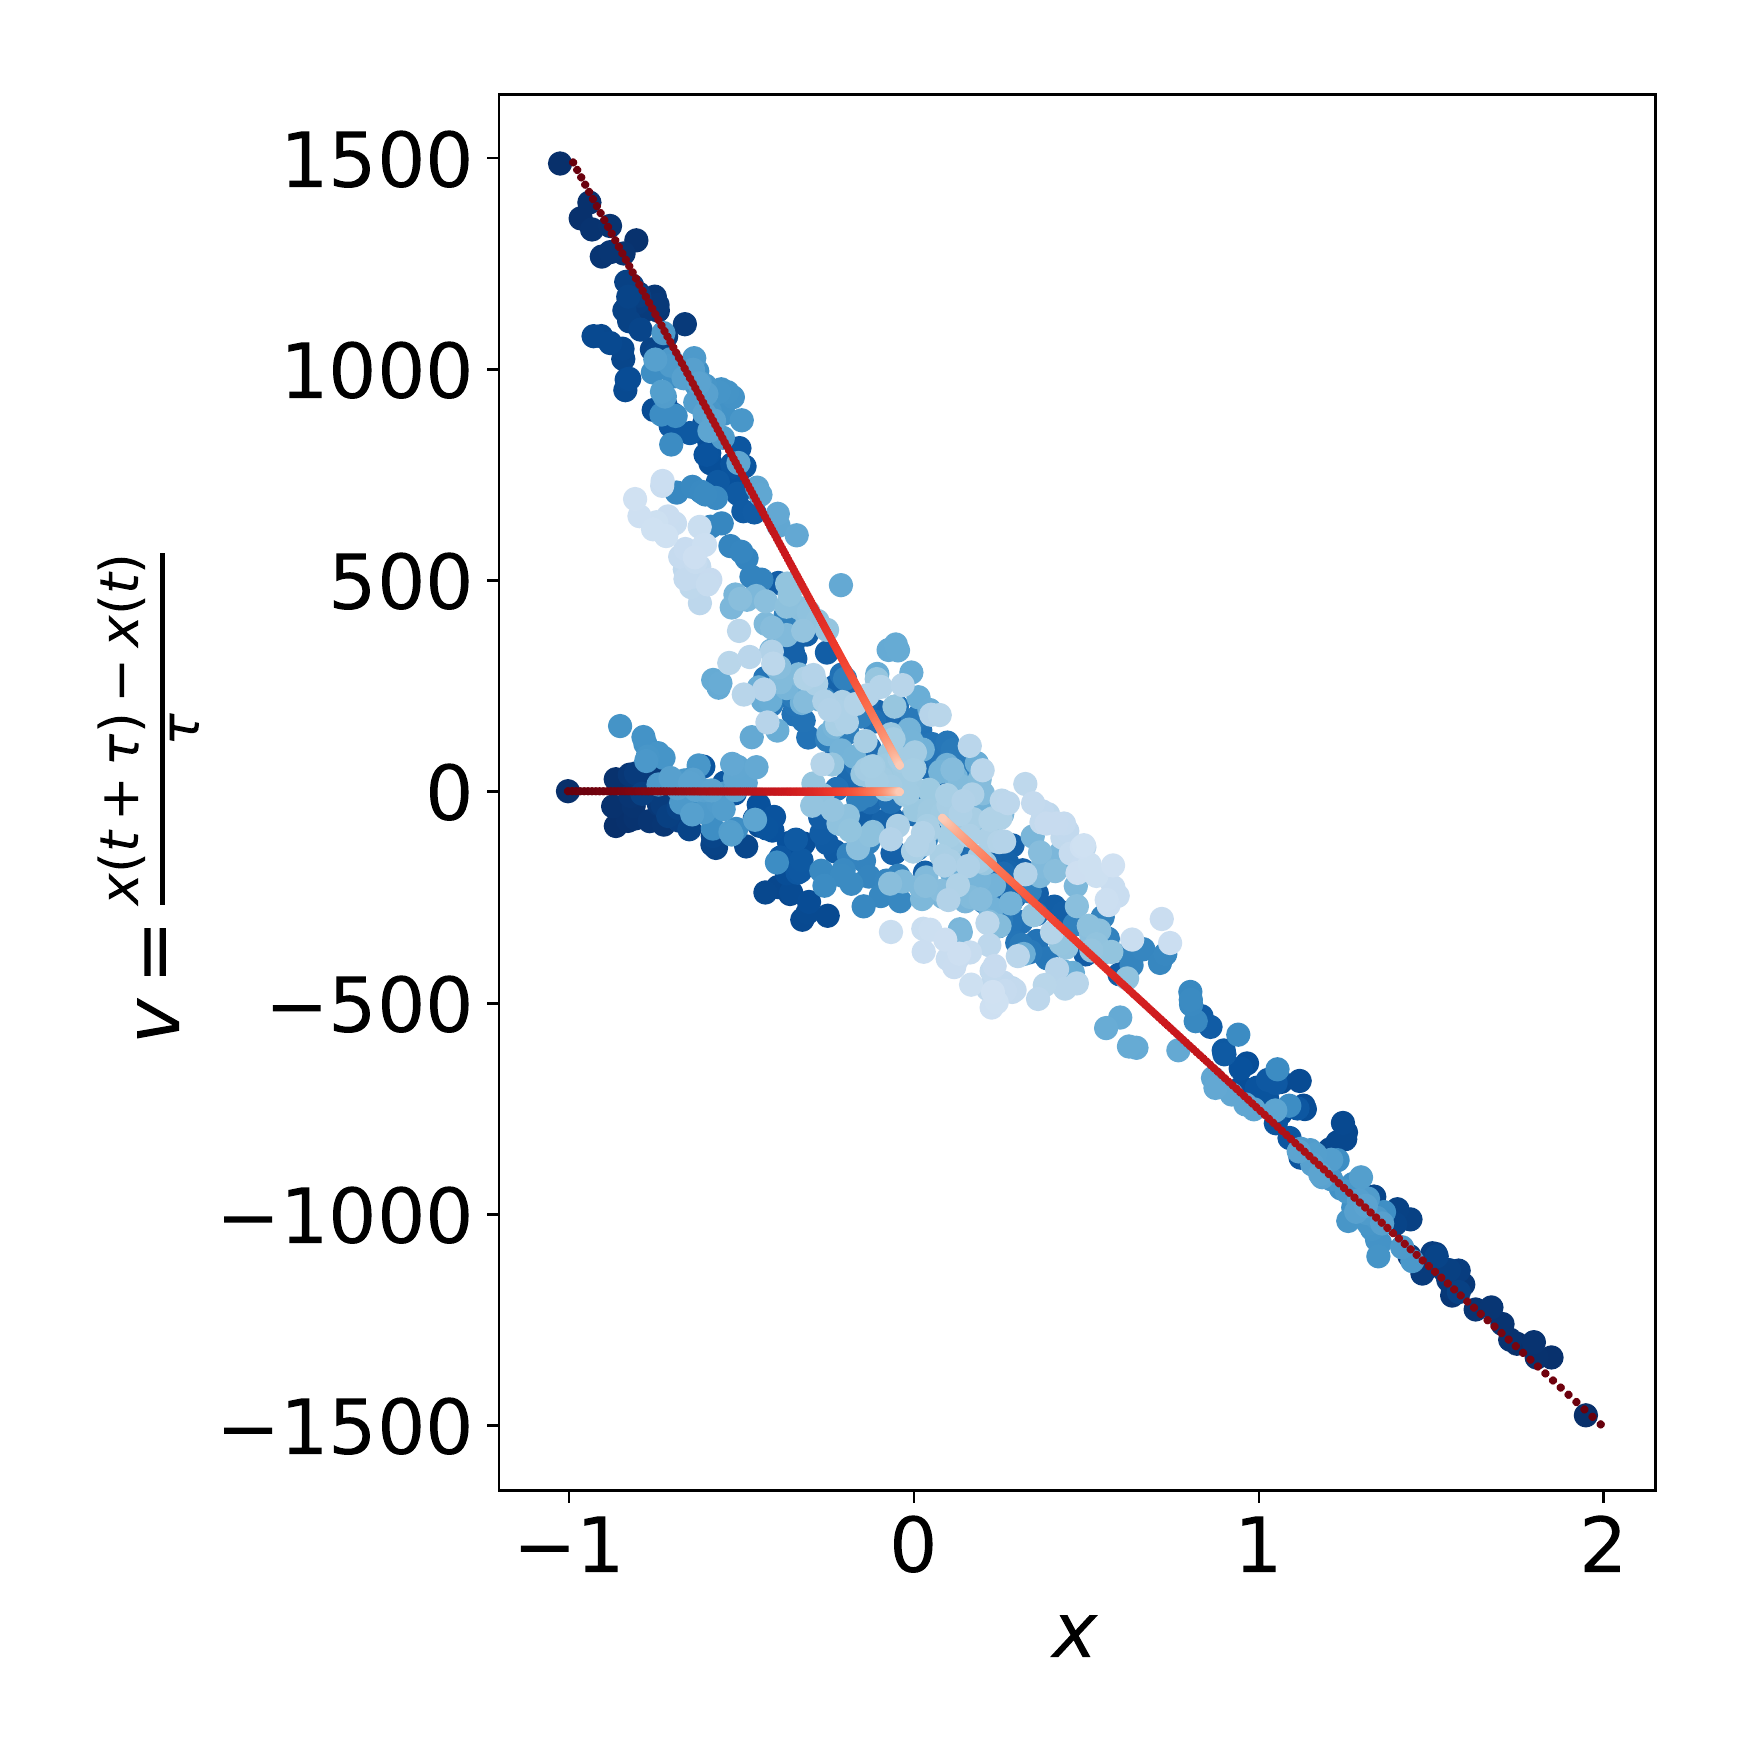}\llap{
  \parbox[b]{1.2cm}{a\\\rule{0ex}{1.97in}}}
\includegraphics[width=.32\columnwidth]{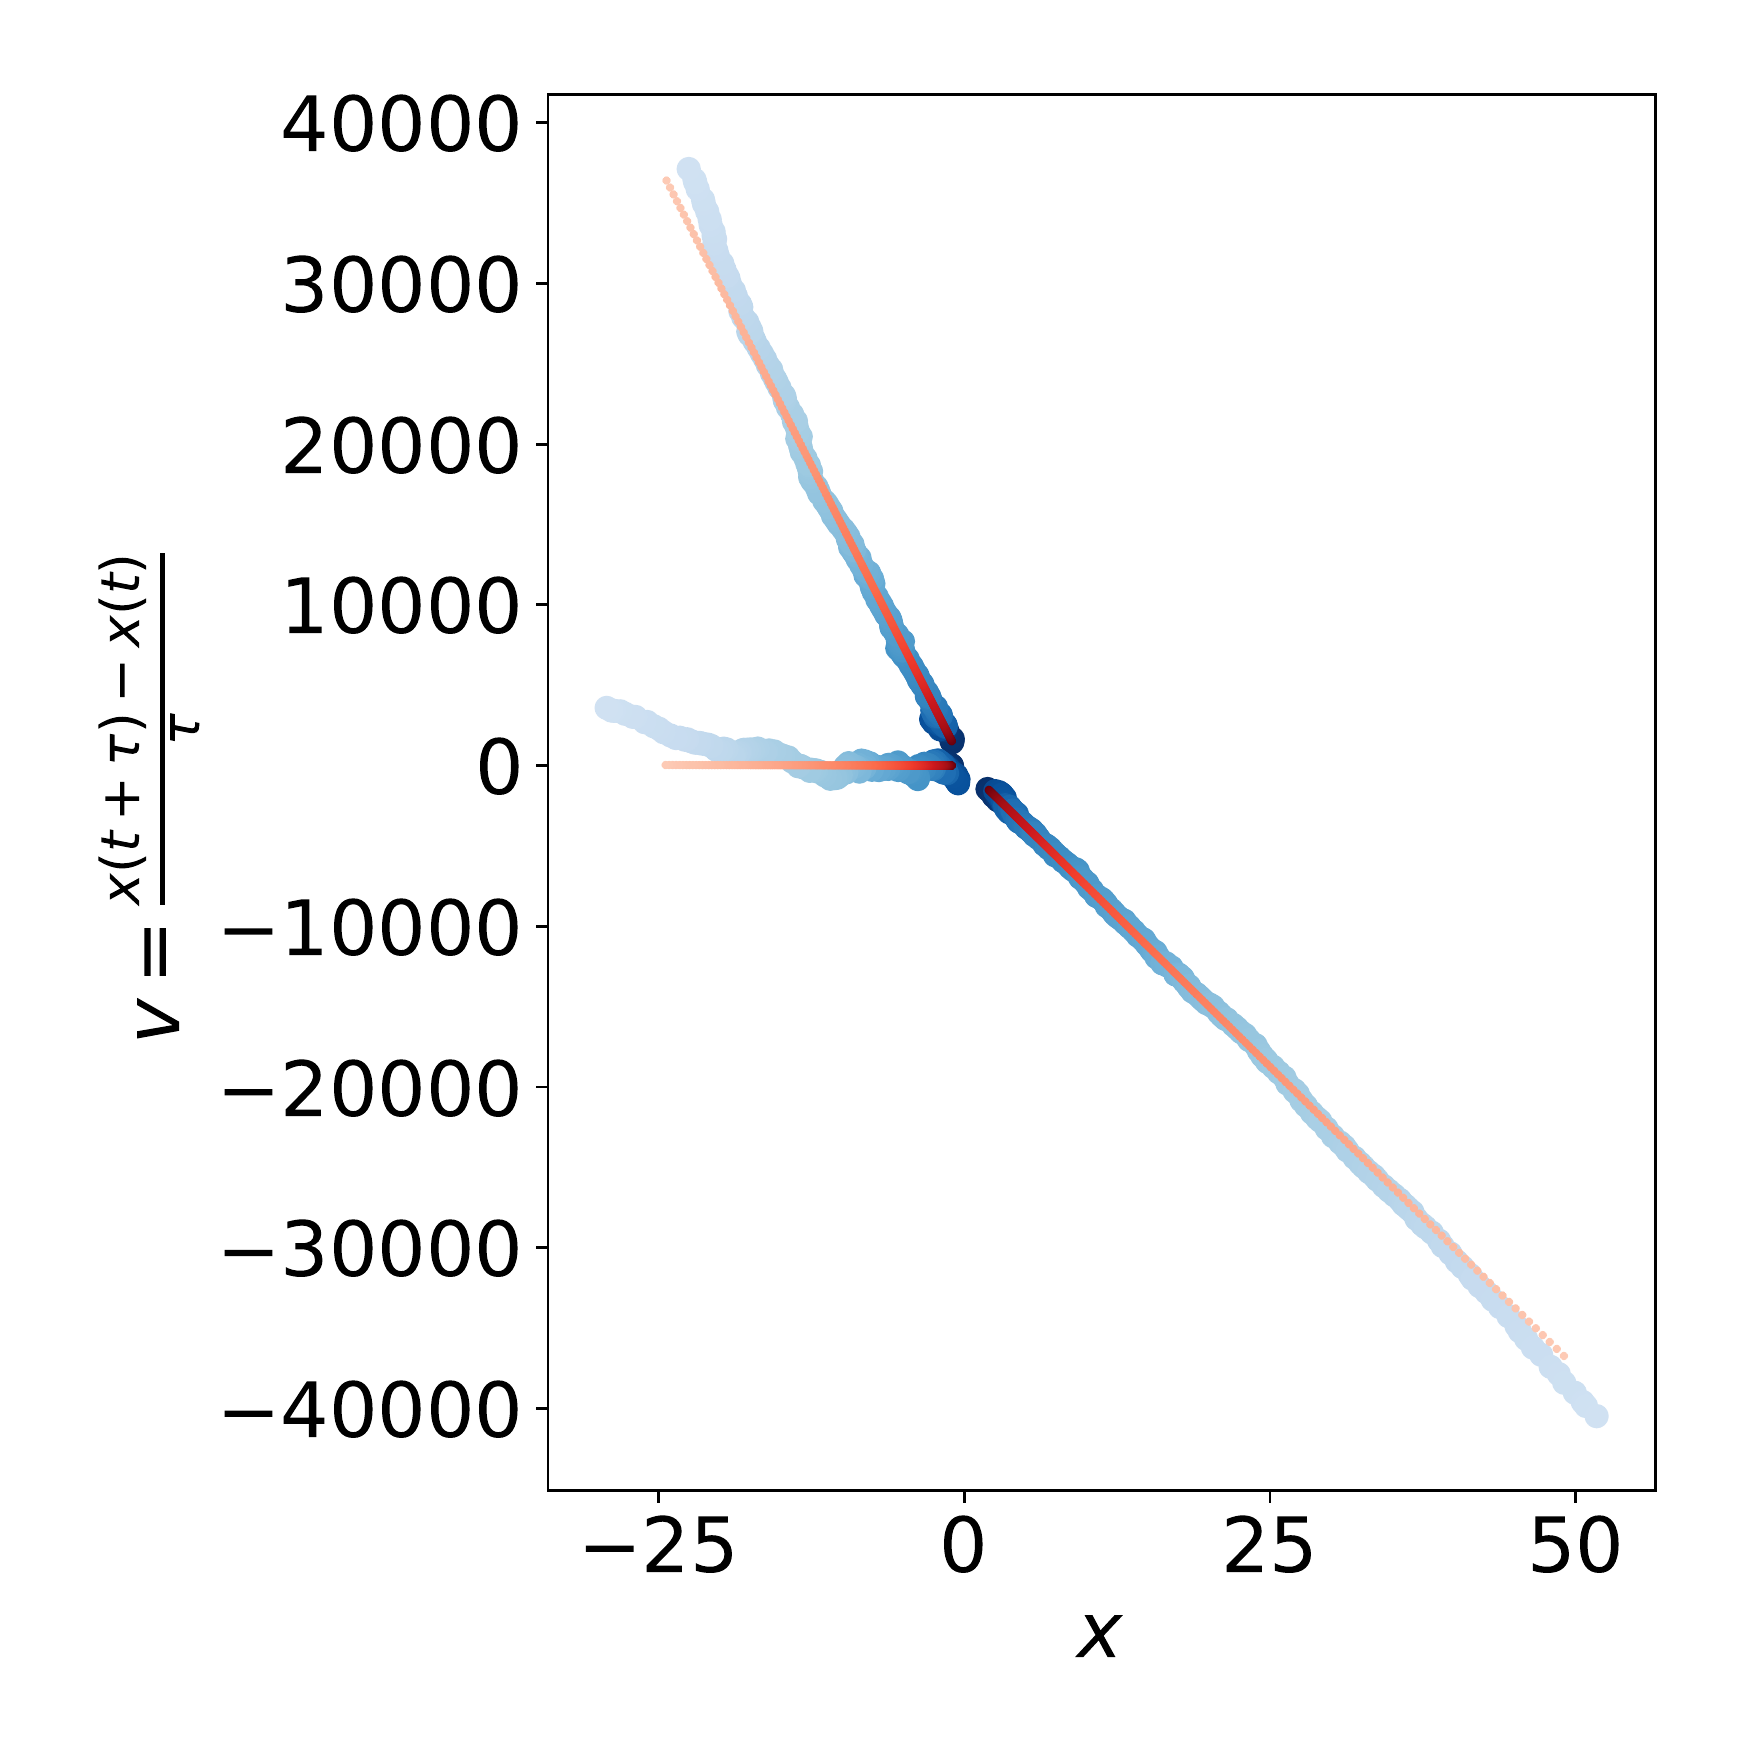}\llap{
  \parbox[b]{1.2cm}{b\\\rule{0ex}{1.97in}}}
\includegraphics[width=.32\columnwidth]{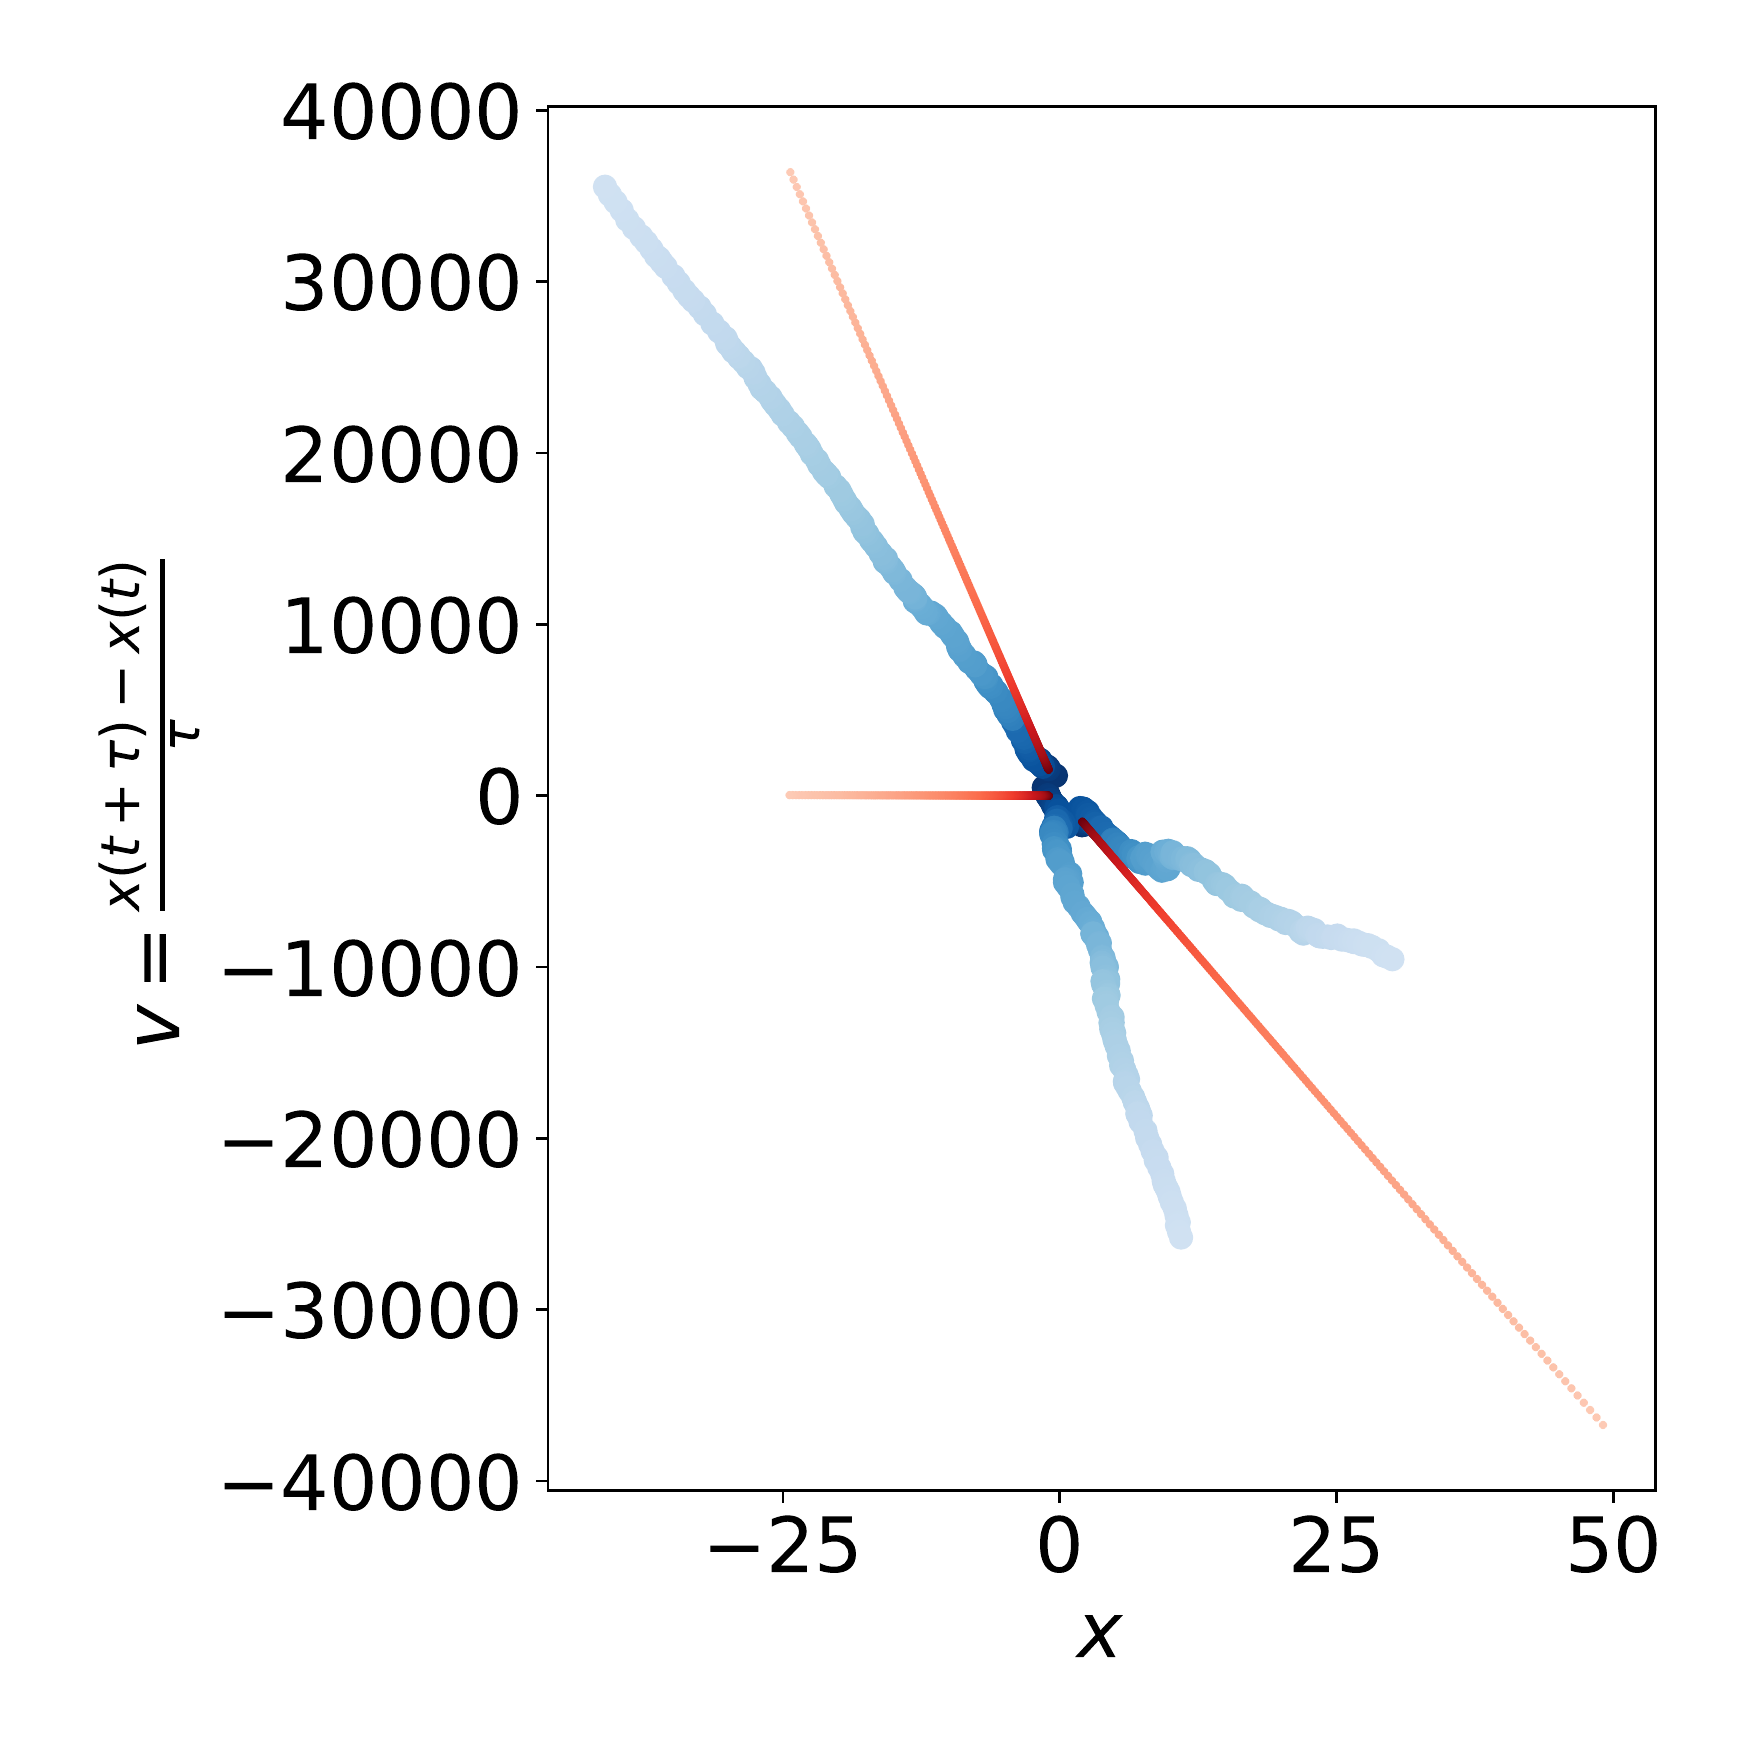}\llap{
  \parbox[b]{1.2cm}{c\\\rule{0ex}{1.97in}}}
\caption{Sample trajectory in the phase diagram of the fixed point process C. Red points are obtained iterating the deterministic process $X_n = \psi X_{n-1}+\theta X_{n-2}$, with $\psi(\tau)=-e^{-\psi_1\tau}$ and $\theta(\tau) = -e^{-2\psi_1\tau}$. Blue points correspond to the stochastic fixed point process, with MA coefficients from Table \ref{tab:MA}. Color code from dark to light indicates advancing time. The deterministic model exhibits a three-branched phase diagram: at each iteration the system jumps from one branch to the next one, moving towards the origin or far from it depending on the modulus of the complex eigenvalues. (a) When $\psi_1>0$ the origin is an asymptotically stable fixed point ($\psi_1=2$, $s=0.5$, $\tau=0.002$). (b-c) The origin becomes unstable for negative $\psi_1$. We plot two samples with parameter values $\psi_1=-2$, $s=2$, $\tau=0.002$. The presence of noise in the unstable case may give rise to very different phase diagrams from the deterministic one, if a large stochastic deviation occurs at small times (cfr Figs. 2b and 2c).}
\label{fig:non-phys}
\end{figure}



\subsection{MA coefficients}

Recurrence relations for the MA coefficients $\mu$ and $\nu$ or, equivalently, for the parameters $\alpha$ and $\beta$, depend on those of the AR coefficients as shown above. The great advantage of working with $\alpha$ and $\beta$ is that, when the AR coefficients are fixed, their recurrence relations are linear: %At any order $k$, the explicit solution is known, as a function of the initial conditions $\alpha_k^{0}, \beta_k^{0}$ and of the coefficient matrix, whose entries depend on $\psi_j^*, \theta_j^*$, for $j\leq k$.
\begin{flalign}
\tilde \alpha_k^{l} &= (1+\psi_0^2+\theta_0^2)\alpha_k^l + 2 \beta_k^l\psi_0(1-\theta_0) + \sum_{i=0}^{k-1} \left[ \alpha_i^l \sum_{j=0}^{k-i} \left(\psi_j\psi_{k-i-j}+\theta_j \theta_{k-i-j}\right)  + 2\beta_i\psi_{k-i}(1-\theta_0) - 2\beta_i\sum_{j=0}^{k-i-1}\psi_j\theta_{k-i-j}\right]\\
\tilde \beta_k^{l} &= \beta_k^l\psi_0(1-\theta_0)-\alpha_k^l\theta_0-\sum_{i=0}^{k-1}\alpha_i^l \theta_{k-i}+\sum_{i=0}^{k-1}\beta_i^l \left[\psi_{k-i}(1-\theta_0)-\sum_{j=0}^{k-i-1}\psi_j\theta_{k-i-j}\right].
\end{flalign}
We analyze their behaviour for each of the 4 fixed points we found for $\psi$ and $\theta$.

\subsubsection*{0th order}
At the leading order we have a homogeneous system
\begin{equation}
\begin{cases}
\alpha_0^{l+1} = \left(1+\psi_0^2+\theta_0^2\right)\alpha_0^{l} + 2\psi_0(1-\theta_0)\beta_0^{l} \\
\beta_0^{l+1} = \psi_0(1-\theta_0)\beta_0^{l} - \theta_0\alpha_0^{l}
\end{cases}
\end{equation}
whose single fixed point is the origin $(\alpha_0^*,\beta_0^*)=(0,0)$, unless the coefficients $\theta_0$ and $\phi_0$ take values that render the fixed point equations linearly dependent. This happens only for the fixed point A, where the condition $(\psi_0^*,\theta_0^*)=(0,0)$ leaves $\alpha_0^*$ as a free parameter, while $\beta_0^*=0$. As a result, $q=0$, and the fixed point model is just a sequence of I.I.D. Gaussian variables. 

For  autoregressive models (i.e. fixed points B-D), the condition $(\alpha_0^*,\beta_0^*)=(0,0)$ tells us that $\tau$-independent noise contributions are prohibited. This feature enables us to interpret these models as discretizations of SDEs corresponding to continuous models \cite{Gardiner}. 

\subsubsection*{1st order}
Moving to a first order expansion (the lowest nontrivial one for the last three fixed points), recursion relations take the form of a 2D affine map:
\begin{equation}
\begin{cases}
\alpha_1^{l+1} = \frac{1}{2}\left\{(1+\psi_0^2+\theta_0^2)\alpha_1^{l} + 2(\psi_0\psi_1 + \theta_0\theta_1)\alpha_0^{l} +2\psi_0(1-\theta_0)\beta_1^{l} + 2\left[\psi_1(1-\theta_0) -\psi_0\theta_1 \right]\beta_0^{l} \right\}\\
\beta_1^{l+1} = \frac{1}{2}\left\{\psi_0(1-\theta_0)\beta_1^{l} + \left[\psi_1(1-\theta_0) -\psi_0\theta_1\right]\beta_0^{l} - \theta_0\alpha_1^{l} - \theta_1\alpha_0^{l} \right\}
\end{cases}.
\end{equation}
Fixed points:
\begin{enumerate}
\item[A.] MA($q$): $(\alpha_0^*,\beta_0^*)=(s,0) \implies (\alpha_1^*,\beta_1^*)=(0,0)$. Even at this order, the process results to be a degenerate MA process, with $q=0$. 
\item[B.] ARMA(1,$q$): $(\alpha_0^*,\beta_0^*)=(0,0) \implies (\alpha_1^*,\beta_1^*)=(s,0)$, with $s$ a real free parameter. As expected, here again $q=0$ and the process reduces to a simple AR(1) model.
\item[C.] ARMA(2,$q$): $(\alpha_0^*,\beta_0^*)=(0,0) \implies (\alpha_1^*,\beta_1^*)=(4s,s)$, $s\in \mathbb R$. We have a manifold of fixed points, represented by a line on the plane of first order covariance coefficients.
\item[D.] AR(I)MA(2,$q$): $(\alpha_0^*,\beta_0^*)=(0,0) \implies (\alpha_1^*,\beta_1^*)=(-2s,s)$. Even in this case, we have a line of fixed point solutions. Interestingly, the corresponding process can be interpreted as the first order discretization of a partially observed Markov process. Suppose that the  measurement consists of a projection onto the $x$ coordinate of the process described by the following set of stochastic differential equations:
\begin{equation}
d\bold y = \bold A \bold y dt + \bold B d\bold W,
\label{general}
\end{equation}
%\begin{flalign}
%\label{x-gen}dx &= vdt + \sigma_xdW_x\\
%\label{v-gen}dv &= -\eta v dt - K x dt + \sigma_vdW_v
%\end{flalign} 
where $\bold W(t)$ is a two-dimensional Wiener process and $\bold A$ and $\bold B\bold B^{\top}$ are the drift and diffusion matrices of the linear SDE. The state variable is here $\bold y=(x,v)$, as we are taking into account two-dimensional systems, but the discussion can be generalized to any $p$-dimensional case. The common assumption is that only the first coordinate $y_1$ of the state variable $\bold y\in \mathbb R^p$ is directly observed. 

When the first row of the $\bold B$ matrix is nonzero, the $x$ process is discretized as an ARMA(2,1) process, even adopting an $O(\tau^{1/2})$ Taylor-It\^o expansion. This fact explains the presence of generally non-null coefficients $\alpha_1$, $\beta_1$ at this order. On the contrary, in the case of purely inertial models, having a singular $\bold B$ matrix with a null first row, the Euler-Maruyama integrator -- corresponding to $O(\tau^{1/2})$ Taylor-It\^o expansion -- yields an AR(2) process. In that case, $\alpha_1=\beta_1=0$, and the first non-null coefficients of the series expansion will appear at the third order. 
%Adopting the generalized Langevin equation formalism: 
%\begin{equation}
%dx(t) = v_0e^{-\eta t}dt+\left[\int_0^t{e^{-\eta(t-s)}f(x(s))\,ds}\right] dt+ \int_0^te^{-\eta(t-s)}\sigma_vdW_v(s) + \sigma_xdW_x(t),
%\label{gen-GL}
%\end{equation}
%it is easier to see that, after removing $v_0$, the process must be discretized as an ARMA(2,1) process and the required minimum order of convergence of the expansion is $O(\tau^{3/2})$. 
A more detailed discussion is postponed to Sec.~\ref{sec:4fp}.
\end{enumerate}

\subsubsection*{2nd order}
Let us write the recurrence relations for second order coefficients 
\begin{dmath}
\begin{cases}
\alpha_2^{l+1} = \frac{1}{4}\big\{(1+\psi_0^2 + \theta_0^2)\alpha_2^{l} + 2(\psi_0\psi_1 + \theta_0\theta_1)\alpha_1^{l} + (2\psi_0\psi_2 + \psi_1^2 +2\theta_0\theta_2+\theta_1^2)\alpha_0^{l} + 2\psi_0(1-\theta_0)\beta_2^{l} + \\
\qquad\quad\ 2\left[\psi_1(1-\theta_0) - \psi_0\theta_1\right]\beta_1^{l} + 2\left[\psi_2(1-\theta_0)-\psi_1\theta_1-\psi_0\theta_2\right]\beta_0^{l}  \big\}\\
\beta_2^{l+1} = \frac{1}{4}\left\{\psi_0(1-\theta_0)\beta_2^{l} + \left[\psi_1(1-\theta_0)-\psi_0\theta_1\right]\beta_1^{l} + \left[\psi_2(1-\theta_0) - \psi_0\theta_2\right]\beta_0^{l} - \theta_0\alpha_2^{l} - \theta_1\alpha_1^{l} - \theta_2\alpha_0^{l} \right\}
\end{cases}
\end{dmath}
and analyze the fixed points:
\begin{enumerate}
\item[A.] MA($q$): $(\alpha_0^*,\beta_0^*,\alpha_1^*,\beta_1^*) = (s,0,0,0) \implies (\alpha_2^*,\beta_2^*)=(0,0)$ i.e. $q=0$ at this order too. 
\item[B.] ARMA(1,$q$): $(\alpha_0^*,\beta_0^*,\alpha_1^*,\beta_1^*) = (0,0,s,0) \implies (\alpha_2^*,\beta_2^*)=\psi_1(s,0)$. The process is still memoryless -- $q=0$ -- as $\beta_2^*=0$, while $\alpha_2^*$ is generally nonzero. Notice, however, that this coefficient is not an arbitrary parameter, but determined by the values of $\psi_1$ and of the lower order coefficient $\alpha_1^*$.
\item[C.] ARMA(2,$q$): $(\alpha_0^*,\beta_0^*,\alpha_1^*,\beta_1^*) = (0,0,4s,s) \implies (\alpha_2^*,\beta_2^*)=-2\psi_1(4s,s)$. As a consequence, the relation between diagonal and off-diagonal entries of the covariance matrix of the random increments is left unchanged going from first to second order: $\alpha_2^*=4\beta_2^*.$
\item[D.] AR(I)MA(2,$q$): $(\alpha_0^*,\beta_0^*,\alpha_1^*,\beta_1^*) = (0,0,-2s,s) \implies (\alpha_2^*,\beta_2^*)=\psi_1(-2s,s)$. As in the previous points, no new free parameter is introduced at this level.
%, the relation between diagonal and off-diagonal entries of the covariance matrix is the same we had at the first order. Moreover, the relation between corresponding first and second order MA coefficients is the same as the AR(1) fixed point, i.e. they are directly proportional through a factor equal to the coefficient $\psi_1$. %\textcolor{red}{maybe it has to do with Strato-Ito diff rules?}
\end{enumerate}

\subsubsection*{3rd order}
We report the recurrence relations for third order coefficients by replacing directly $\beta_0^{l}=0$:
\begin{equation}
\begin{cases}
\alpha_3^{l+1} = \frac{1}{8}\big\{(1+\psi_0^2 + \theta_0^2)\alpha_3^{l} + 2(\psi_0\psi_1 + \theta_0\theta_1)\alpha_2^{l} + (2\psi_0\psi_2 + \psi_1^2 +2\theta_0\theta_2+\theta_1^2)\alpha_1^{l} + 2(\psi_0\psi_3 + \psi_1\psi_2 + \theta_3\theta_0 \\
\qquad\quad\quad\  + \theta_1\theta_2)\alpha_0^{l} +2\psi_0(1-\theta_0)\beta_3^{l} + 2\left[\psi_1(1-\theta_0) - \psi_0\theta_1\right]\beta_2^{l} + 2\left[\psi_2(1-\theta_0)-\psi_1\theta_1-\psi_0\theta_2\right]\beta_1^{l}\\
%+2\left[\psi_3(1-\theta_0)- \psi_2\theta_1 -\psi_1\theta_2-\psi_0\theta_3\right]\beta_0^{l} \big\}\\
\beta_3^{l+1} = \frac{1}{8}\left\{\psi_0(1-\theta_0)\beta_3^{l} + \left[\psi_1(1-\theta_0)-\psi_0\theta_1\right]\beta_2^{l} + \left[\psi_2(1-\theta_0) - \psi_0\theta_2\right]\beta_1^{l} - \theta_0\alpha_3^{l} - \theta_1\alpha_2^{l} - \theta_2\alpha_1^{l} - \theta_3^{l}\alpha_0^{l} \right\}.
\end{cases}
\label{MA3-rec}
\end{equation}
Fixed points:
\begin{enumerate}
\item[A.] MA($q$): $(\alpha_0^*,\beta_0^*,\alpha_1^*,\beta_1^*,\alpha_2^*,\beta_2^*) = (s,0,0,0,0,0) \implies (\alpha_3^*,\beta_3^*)=(0,0)$. The unique stable fixed point is just a sequence of random I.I.D. Gaussian variables.
\item[B.] ARMA(1,$q$): $(\alpha_0^*,\beta_0^*,\alpha_1^*,\beta_1^*,\alpha_2^*,\beta_2^*) = (0,0,s,0,\psi_1s,0) \implies (\alpha_3^*,\beta_3^*)=(\frac{2}{3}\psi_1^2s,0)$. Even at this order, the process is an AR(1) model, without memory nor color. It is proven by induction that this holds true at any subsequent order.
\item[C.] ARMA(2,$q$): $(\alpha_0^*,\beta_0^*,\alpha_1^*,\beta_1^*,\alpha_2^*,\beta_2^*) = (0,0,4s,s,-8\psi_1s,-2\psi_1s) \implies (\alpha_3^*,\beta_3^*)=(\frac{32}{3}\psi_1^2s,\frac{13}{6}\psi_1^2s)$. The relation between diagonal and off-diagonal entries of the covariance matrix of random increments is different from the one we had at lower orders, but no new free parameter is introduced.
\item[D.] AR(I)MA(2,$q$): $(\alpha_0^*,\beta_0^*,\alpha_1^*,\beta_1^*,\alpha_2^*,\beta_2^*) = (0,0,-2s,s,-2\psi_1s,\psi_1s) \implies (\alpha_3^*,\beta_3^*)=(4b-(2\psi_2+3\psi_1^2)s,b)$. For this nontrivial fixed point, the recurrence relations in Eq.~\eqref{MA3-rec} are linearly dependent, and admit infinitely many solutions. We parametrize them by taking $\beta_3^*=b$. The additional arbitrariness we find at this order is easily explained if we consider this fixed point model as a discretized underdamped Langevin equation. The presence of a dynamical noise source acting on the unobserved degree of freedom $v$ results into an $O(\tau^3)$ contribution for the covariance matrix entries, which is independent of the previous $O(\tau)$ contribution. A broader discussion about this fourth fixed point of physical interest can be found in Sec.~\ref{sec:4fp}.

%%%%%%%%
%Following \cite{Zwanzig_book,LI}, one should firstly integrate Eq.\eqref{gen-GL} over the intervals $[0,\tau]$ and $[\tau,2\tau]$ and linearly combine the resulting equations in order to cancel the $v_0$ term:
%\begin{dmath}
%x(2\tau)-(1+e^{-\eta\tau})x(\tau) + e^{-\eta\tau} x(0) = \int_0^{2\tau}  \psi(s-\tau)  f\left(x(s)\right) ds + \int_0^{2\tau} \psi(s-\tau)  \sigma_v dW_v(s) + \int_{\tau}^{2\tau} \sigma_x dW_x(s) - e^{-\eta\tau}\int_{0}^{\tau}\sigma_x dW_x(s),
%\label{eq:update}
%\end{dmath}  
%where
%\begin{equation}
%\psi(s)=
%\begin{cases}
%\frac{e^{\eta s}-e^{-\eta\tau}}{\eta}\quad \text{for } -\tau<s<0\\
%\frac{1-e^{\eta(s-\tau)}}{\eta} \quad \text{for } 0<s<\tau.
%\end{cases}
%\end{equation}

%Notice that, since $x(s)$ is a stochastic process, the first term of the r.h.s. is contributing, in general, to the definition of the noise increment of the discrete-time update equation. This fact explains the presence of $z$ in Table \ref{tab:MA}. However, when $\sigma_x=0$, this contribution si only affecting coefficients of higher order than $\alpha_3$ and $\beta_3$. It is instructive to check that computing the covariance entries from Eq.~\eqref{eq:update} would provide the same results we obtained as fixed point solutions of the recurrence relations.



%We define the random increment associated to the update equation at the $n$-th step as
%\begin{equation}
%r_n = \int_{t_n-2\tau}^{t_n}\psi(s-\tau)\sigma_v  dW_v(s) + \int_{t_n-2\tau}^{t_n -\tau} \sigma_x dW_x(s) - e^{-\eta\tau}\int_{t_n-\tau}^{t_n}\sigma_x dW_x(s)
%\end{equation}
%The probability density  are specified by 
%\begin{equation}
%\Exp{r_n^2}
%\end{equation}

\end{enumerate}

Table \ref{tab:MA} summarizes the findings related to the MA coefficients of the 4 fixed points. Notice that, in addition to the reported 4 fixed points, there is also the diverging fixed point, having $\psi_k^*=\theta_k^*=\infty$, $\alpha_k^*=\beta_k^*=\infty$ $\forall k$.
\begin{table}[h] 
\caption{\label{tab:MA} 
Fixed points -- MA coefficients. Fixed point models are reported in the same order as in Table \ref{tab:AR}, specifying here the moving average order associated to each. We denote $u=\psi_1^*$, $z=\psi_2^*$.
}
\begin{ruledtabular}
\begin{tabular}{c c c c  c c  c c  c c }
\centering
&Model & $\alpha_0^*$ & $\beta_0^*$ & $\alpha_1^*$ & $\beta_1^*$ & $\alpha_2^*$ & $\beta_2^*$ & $\alpha_3^*$ & $\beta_3^*$ \\

A. &  MA(0) & $s$ & 0 & 0 & 0 & 0 & 0 & 0 & 0\\
B. & AR(1) & 0 & 0 & $s$ & 0 & $us$ & 0 & $2u^2s/3$ & 0 \\
C. & ARMA(2,1) & 0 & 0 & $4s$ & $s$ & $-8us$ & $-2us$ & $32u^2s/3$ & $13u^2s/6$\\
D. & AR(I)MA(2,1) & 0 & 0 & $-2s$ & $s$ & $-2us$ & $us$ & $4b - (2z+3u^2)s$ & $b$\\
\end{tabular}
\end{ruledtabular}
\end{table}

Induction can be applied also to the recursion relations of the MA coefficients to show that the nature of the fixed points is left unchanged if one takes higher order expansions. In particular, one can prove that 
\begin{enumerate}
\item Fixed point A is a pure random sequence of IID Gaussian variables. The only non-null parameter is $\alpha_0$, while $\beta_k=0$ and $\alpha_j=0$ for any $k\geq0$ and $j\geq1$.
\item Fixed point B is at any order a simple autoregressive process of order one, AR(1), since $\beta_k=0$ $\forall k$. The variance of the random increment is reconstructed as the series expansion with coefficients $\alpha_0=0$, $\alpha_k = \alpha_1\frac{(2\psi_1)^{k-1}}{k!}$ for $k\geq1$. Hence, $\alpha(\tau)=\frac{\alpha_1}{2\psi_1}\left(e^{2\psi_1\tau}-1\right)$.
\end{enumerate}


%%%%%%%%%%%%%%%%%%%%%%%%%%%%%%%%%%%%%%%%%%%%%%%%%%%%%%%%%%%%%%
%%%%%%%%%%%%%%%%%%%%%%%%%%%%%%%%%%%%%%%%%%%%%%%%%%%%%%%%%%%%%%
\section*{III. The fourth fixed point}\label{sec:4fp}

This section is devoted to a more detailed discussion of the fourth fixed point, which, due to its physical meaning, we think deserves a special focus. 
We have already highlighted that, at leading order, the AR coefficients reproduce a second time derivative through the double differencing operator $\Delta^2=(1-L)^2$, with $L$ the lag operator: $LX_n = X_{n-1}$. This fact gives to the model an `integrated process' nature at leading order, also known as ARIMA(1,1,1) \cite{Brockwell-Davis-book}. Since the relation 
\begin{equation}
	\lim_{\tau\to0}\frac{\psi-\psi_0^*}{\tau} = -\lim_{\tau\to0}\frac{\theta-\theta_0^*}{\tau}
\end{equation}
also holds, this integrated process structure is kept up to $O(\tau)$. Deviations from it occur at higher order and are due to the presence of linearly $x$-dependent forces. 

The fixed point model is indeed the consistent discretization of a general class of partially observed continuous-time processes described by Eq.~\eqref{general}:
\begin{equation}
d\bold y = \bold A \bold y dt + \bold B d\bold W,
\label{general-2}
\end{equation}
where 
\begin{equation}
\bold y = (x,v)^{\top}, \quad \bold W = (W_x,W_v)^{\top}
,\quad \bold A = \begin{pmatrix}
-\lambda & 1 \\
-\kappa & -\eta
\end{pmatrix}, \quad \bold B \bold B^{\top}= \begin{pmatrix}
\sigma_{xx}^2 & \sigma_{xv}^2 \\
\sigma_{vx}^2 & \sigma_{vv}^2 
\end{pmatrix}. 
\label{param}
\end{equation}
$W_x(t)$ and $W_v(t)$ are independent Wiener processes. Notice that setting $A_{12}=1$ does not imply a loss of generality: compared to $A_{12}=a\in \mathbb R\setminus\{0\}$, it just corresponds to a rescaling of the time unit, which does not alter the process (the only caveat is that $a<0$ would revert the time direction). The case $A_{12}=0$ is not of interest for us, as it would decouple the dynamics of the unobserved degrees of freedom from that of the observed ones. The entries in the drift matrix $\bold A$ must satisfy the stability condition, i.e., assuming that time evolves in the positive direction, $t\in [0,\infty[$, that it is negative semidefinite part. Finally, $\sigma_{xv}^2=\sigma_{vx}^2$ for the symmetry of the diffusion matrix.

Partial observation of the process in Eq.~\eqref{general-2} is a Gaussian process described, at the continuous level, by a Generalized Langevin Equation (GLE), and, at the discrete level, by an ARMA(2,1) model. The GLE can be obtained by integrating the equation for the $v$ variable and plugging it into the first one in \eqref{general-2}:
\begin{equation}
dx(t) = \left\{e^{-\eta t} v(0) - \kappa \int_0^t dt' e^{-\eta(t-t')}x(t') + \int_0^t \left[B_{21}dW_x(t') + B_{22}dW_v(t')\right]\right\}dt - \lambda x(t) + B_{11}dW_x(t)+ B_{12}dW_v(t).
\label{GLE-gen}
\end{equation}
This equation contains a parametric dependence on the initial condition $v(0)$, which we wish to eliminate. As in \cite{LI, prx}, one can self-consistently do it to obtain an approximate ARMA(2,1) model which only depends on the inertial coordinates. An alternative way to do it (without approximations, thanks to linearity) is to restart from the exact integration of Eq.\eqref{general-2}:
\begin{equation}
\bold y(t) = e^{\bold A (t-t_0)}\bold y(t_0) + \int_{t_0}^t e^{\bold A(t-s)}\bold B d\bold W(s)
\label{integral}
\end{equation}
and to linearly combine the first components of $\bold y(t_n)$ and $\bold y(t_n - \tau)$ to obtain:
\begin{equation}
X_n - \frac{\left(e^{2\bold A\tau}\right)_{12}}{\left(e^{\bold A\tau}\right)_{12}}X_{n-1} - \left[ \left(e^{2\bold A\tau}\right)_{11} - \frac{\left(e^{2\bold A\tau}\right)_{12}}{\left(e^{\bold A\tau}\right)_{12}}\left(e^{\bold A\tau}\right)_{11} \right] X_{n-2}  =  r_n,
\label{exact-discr}
\end{equation}
with 
\begin{dmath}
r_n = \int_{t_n-2\tau}^{t_n} \left(e^{\bold A(2\tau-s)}\right)_{11}\left[B_{11}dW_x(s) + B_{12}dW_v(s)\right] - \frac{\left(e^{2\bold A\tau}\right)_{12}}{\left(e^{\bold A\tau}\right)_{12}} \int_{t_n-2\tau}^{t_n-\tau}  \left(e^{\bold A(\tau-s)}\right)_{11}\left[B_{11}dW_x(s) + B_{12}dW_v(s)\right] + 
\int_{t_n-2\tau}^{t_n} \left(e^{\bold A(2\tau-s)}\right)_{12}\left[B_{21}dW_x(s) + B_{22}dW_v(s)\right] - \frac{\left(e^{2\bold A\tau}\right)_{12}}{\left(e^{\bold A\tau}\right)_{12}} \int_{t_n-2\tau}^{t_n-\tau}  \left(e^{\bold A(\tau-s)}\right)_{12}\left[B_{21}dW_x(s) + B_{22}dW_v(s)\right].
\label{rn}
\end{dmath}
Eq.~\eqref{exact-discr} corresponds to an ARMA(2,1) process, since Eq.\eqref{rn} implies that $\Exp{r_nr_m}=\alpha \delta_{n,m} + \beta \delta_{n,m\pm1}$. It is possible to explicitly work out the calculation to find the (noninvertible) mapping between $(\bold A,\bold B\bold B^{\top})$ and $(\psi,\theta,\alpha,\beta)$.

In order to associate the parameters of the fixed point D in Tables \ref{tab:AR} and \ref{tab:MA} to the physical parameters of the process in Eq.~\eqref{param}, it is convenient to perform a small $\tau$ expansion of the equations mapping $(\bold A,\bold B\bold B^{\top})$ to $(\psi,\theta,\alpha,\beta)$. Consider the AR coefficients first:
%
\begin{flalign}
\label{psi_map} \psi &= \frac{\left(e^{2\bold A\tau}\right)_{12}}{\left(e^{\bold A\tau}\right)_{12}} %\simeq 2+\tau \left(A^2\right)_{12} + \tau^2\left[\left(A^3\right)_{12} - \frac{1}{2} \left(A^2\right)^2_{12}\right] + \tau^3\left[\frac{7}{12}\left(A^4\right)_{12} - \frac{2}{3}\left(A^2\right)_{12}\left(A^3\right)_{12} + \frac{1}{4}\left(A^2\right)^3_{12}\right]
\simeq 2- (\eta+\lambda)\tau + \frac{1}{2}\tau^2\left(-2\kappa+\eta^2+\lambda^2\right) + \frac{1}{6}\tau^3\left(3\kappa(\eta+\lambda)-\eta^3-\lambda^3\right);
\\
\label{theta_map} \theta &= \left(e^{2\bold A\tau}\right)_{11} - \frac{\left(e^{2\bold A\tau}\right)_{12}}{\left(e^{\bold A\tau}\right)_{12}}\left(e^{\bold A\tau}\right)_{11} = -e^{-(\eta+\lambda)\tau}\simeq
-1 + (\eta+\lambda)\tau - \frac{1}{2}\tau^2(\eta+\lambda)^2 + \frac{1}{6}(\eta+\lambda)^3.
%\simeq -1 - \tau \left(A^2\right)_{12} + \tau^2 \left[\left(A^2\right)_{11} - \left(A^2\right)_{12}A_{11} - \left(A^3\right)_{12} + \frac{1}{2}\left(A^2\right)^2_{12}\right] + \tau^3\left[ \left(A^3\right)_{11} - \left(A^3\right)_{12}\left(A_{11}+\frac{1}{2}\left(A^2\right)_{12}\right) - \frac{1}{3}\left(A^2\right)^3_{12} + \frac{1}{2} \left(A^2\right)^2_{12}A_{11} - \frac{1}{2} \left(A^2\right)_{12}\left(A^2\right)_{11}\right].
\end{flalign}
%
Identifying the coefficients  $\psi_0\dots\psi_3$ and $\theta_0\dots\theta_3$, one can deduce that the model parameters in Eq.~\eqref{param} and the fixed point parameters of process D in Table~\ref{tab:AR} are linked by the following relation:
\begin{equation}
u = -(\lambda+\eta); \quad z = -\kappa + \frac{1}{2}(\eta^2+\lambda^2).
\label{map-AR}
\end{equation}
The algebra for the derivation of $\alpha$ and $\beta$ is more laborious but not complicated. The results are as follows:
\begin{flalign}
\alpha &\simeq 2\sigma_{xx}^2\tau - 2\sigma_{xx}^2(\eta+\lambda)\tau^2 + \frac{2}{3}\left[\sigma_{vv}^2+2\eta\sigma_{xv}^2+\sigma_{xx}^2(-\kappa+3\eta^2+3\eta\lambda+2\lambda^2)\right]\tau^3;\\
\beta &\simeq -\sigma_{xx}^2\tau + \sigma_{xx}^2\tau^2 + \frac{1}{6}\left[\sigma_{vv}^2 + 2\eta\sigma_{xv}^2 + \sigma_{xx}^2(2\kappa-3\eta^2-6\eta\lambda-4\lambda^2)\right]\tau^3.
\end{flalign}
Hence we can deduce:
\begin{equation}
s=-\sigma_{xx}^2; \quad b = \frac{1}{6}\left[\sigma_{vv}^2 + 2\eta\sigma_{xv}^2 + \sigma_{xx}^2(2\kappa-3\eta^2-6\eta\lambda-4\lambda^2)\right].
\label{map-MA}
\end{equation}

In summary, we have showed that the fixed point solutions of the real space RG map defined above for ARMA(2,1) time series are the exact discretizations of second order linear SDEs. These models represent a special class of Gaussian processes with a clear continuous-time interpretation. 

Notice that the mapping given by Eqs.~\eqref{map-AR} and \eqref{map-MA} is noninvertible. Because of the partial nature of the observation, multiple models are mapped to the same ARMA process. In other words, there is no bijection between the continuous-time Markovian description of the dynamical system and its experimental non-Markovian observation. A unique reconstruction of a set of first order SDEs is impossible. Extracting the parameters of an underlying continuous-time Markov model from time series analysis is therefore an arbitrary task, which postulates the choice of suitable hidden variables. Without loss of generality, one can therefore reduce the number of parameters to 4 by setting $\lambda=0$, $\sigma_{xv}^2=0$. 

\subsubsection*{Inertial processes}
A subclass of models contained in fixed point D is represented by inertial processes, which take the form:
\begin{flalign}
dx &= vdt;\\
dv &= -\eta v dt - \kappa x dt +\sigma_{vv}dW_v.
\label{inertial-ex}
\end{flalign}
They are obtained by setting $\lambda=\sigma_{xv}^2=0$ (which does not change the nature of the process) and $\sigma_{xx}^2=0$. This condition implies that there are no $O(\tau^{1/2})$ stochastic contributions to the observed process; results can be read from Table \ref{tab:MA} setting $s=0$. Because of the absence of $O(\tau^{1/2})$ stochastic contributions, applying a Euler-Maruyama discretization to purely inertial models gives rise to an AR(2) model. 
%On the contrary, when $\sigma_x\neq0$ adopting a Euler-Maruyama scheme yields an (inconsistent) ARMA(2,1) model. 

We can take this inconsistent discretization of the 2nd order SDE as an initial condition for the RG recurrence relations of MA coefficients.
Since $s=0$, we have null $\alpha_k$ and $\beta_k$ up to $k=3$. Third order recurrence relations are in this case:
\begin{equation}
\begin{cases}
\alpha_3^{l+1} = \frac{1}{8}\left[6\alpha_3^{l}+8\beta_3^{l}\right]\\
\beta_3^{l+1} = \frac{1}{8}\left[\alpha_3^{l}+4\beta_3^{l}\right].
\end{cases}
\label{inertial-rec-3}
\end{equation}
Orbits are lines in the $(\alpha_3,\beta_3)$ plane: $\alpha_3+2\beta_3=c$, being $c$ a constant fixed by the initial condition $(\alpha_3^{0},\beta_3^{0})=(\sigma_{vv}^2,0)$. The intersection with the line of fixed points, $\alpha_3^*=4\beta_3^*$, identifies, in our space of parameters, the model which is reached by repeatedly coarse-graining the starting discrete-time model. An illustration is in Fig.\ref{fig:rec_rel}b.
Thanks to linearity, one can also compute how the asymptotic point is approached. The solution of Eq.~\eqref{inertial-rec-3} is
\begin{equation}
\begin{cases}
\alpha_3^{l} = 4^{-l}\frac{1}{3}\left[\alpha_3^{0}-\beta_3^{0}\right]+\frac{2}{3}\left[\alpha_3^{0}+2\beta_3^{0}\right]\\
\beta_3^{l} = 4^{-l}\left[\frac{2}{3}\beta_3^{0}-\frac{1}{6}\alpha_3^{0}\right]+\frac{1}{6}\left[\alpha_3^{0}+2\beta_3^{0}\right].
\end{cases}
\label{sol-ab-3}
\end{equation}
 Under subsequent iterations of the RG procedure, the covariance matrix of random increments, $C^l_{nm}=\Exp{r_n^lr_m^l}$, is modified as follows:
\begin{equation}
C^{0}=\sigma_{vv}^2
	\begin{pmatrix}
	1 & 0 & \dots & 0\\
	0 & 1 & . & \vdots\\
	\vdots & . & \ddots & 0\\
	0 & \dots & 0 & 1
	\end{pmatrix}
	\longrightarrow
	C^{1}=\sigma_{vv}^2\begin{pmatrix}
	3/4 & 1/8 & \dots & 0\\
	1/8 & 3/4 & . & \vdots\\
	\vdots & . & \ddots & 1/8\\
	0 & \dots & 1/8 & 3/4
	\end{pmatrix}
	\longrightarrow
	\dots
	\longrightarrow
	C^{\infty}=\sigma_{vv}^2\begin{pmatrix}
	2/3 & 1/6 & \dots & 0\\
	1/6 & 2/3 & . & \vdots\\
	\vdots & . & \ddots & 1/6\\
	0 & \dots & 1/6 & 2/3
	\end{pmatrix}.
	\label{matrix-step1}
\end{equation}
Asymptotically, it converges to the covariance matrix of a consistent $O(\tau^{3/2})$ integration scheme. This fact justifies that, despite the order of strong convergence of the Euler scheme is $1/2$ and it yields inconsistencies when adopted for inferring second-order SDEs, observing the simulated process at a scale much larger than the simulation step makes it acquire an effective higher order of convergence. In other words, infinitely many Euler integration steps within a given time interval are equivalent to a single integration step on that interval performed using an integration scheme which is strongly convergent at least as $\tau^{3/2}$.
There is then an `asymptotic upgrade' of the order of convergence of the scheme, at least in the linear case. We don't know to what extent this is extendible to the nonlinear case, since stability issues of the scheme may be relevant. It is however clear that nonlinear discrete white noise models resulting from Euler discretizations are still inappropriate. However, reliable numerical integrators are available, like \cite{LI}, which has been used in \cite{prx} to develop a Bayesian inference scheme for underdamped Langevin models.


%%%%%%%%%%%%%%%%%%%%%%%%%%%%%%%%%%%%%%%%%%%%%%%%%%%%%%%%%%%%%%
%%%%%%%%%%%%%%%%%%%%%%%%%%%%%%%%%%%%%%%%%%%%%%%%%%%%%%%%%%%%%%
\section*{IV. Effective AR(2) models for partially observed Langevin equations at equilibrium}\label{sec:AR2}

The argument we presented so far is not based on any stationarity nor equilibrium assumption for the continuous process we observe. It only relies on the requirement that the discretized model must have an invariant structure under coarse graining. Such a requirement ensures that a transition over a time interval $2\tau$ can be equivalently described, up to a given order of approximation, either by a discretization on a single time step of amplitude $2\tau$ or by the composition -- using the same scheme -- of two $\tau$-steps. 
When this request is not satisfied, the discretization is inadequate, producing biased estimators when applied to inference problems \cite{Pedersen,GloterOU,prx}. Given a damped Langevin equation like
\begin{flalign}
\label{eq-xv-1}	d x &= v dt;\\ 
\label{eq-xv-2}	d v &= \left[-\eta v - \kappa x \right]dt + \sqrt{2T\eta} dW,
\end{flalign}
the bias comes in the form of a $\tau$-independent rescaling factor equal to 2/3 for the linear damping coefficient $\eta$, whereas the remaining parameters are unbiasedly estimated. 

How universal is this behaviour? We conjecture that the inconsistency of the inference scheme is absorbed by such a simple rescaling for all inertial equilibrium processes (described by generalizations of Eqs.~\eqref{eq-xv-1}--\eqref{eq-xv-2}, obtained replacing the elastic force with any conservative $f(x)$), also known as Kramers processes. In this section we try to provide an argument for this fact, working out the reference problem of an integrated Ornstein-Uhlenbeck (OU) process. 

The integrated OU process is the simplest example of 2nd-order SDE for which the Euler-related inconsistency appears. It is described by the Eqs.~\eqref{eq-xv-1}--\eqref{eq-xv-2} with $\kappa=0$. Suppose we can only observe (with infinite accuracy) the inertial degree of freedom, at a sampling rate $\tau^{-1}$. 
%\begin{equation}
%	dx = vdt;\;\ dv = -\eta v dt + \sigma dW.
%	\label{OU}
%\end{equation}
Let us recall the notation for the time series of empirical observations $\{X_n\}_{n\in \mathbb N}$, and for that of reconstructed velocities $\{\bar V_n\}_{n\in \mathbb N}$, where 
\begin{equation}
\bar V_n = \frac{\left(X_{n+1}-X_n\right)}{\tau}.
\end{equation}
Let us also introduce the series of \emph{real} velocities $\{V_n\}_{n\in \mathbb N}$, corresponding to the one we would obtain if we were able to measure directly the velocity degree of freedom. Because the evolution of this degree of freedom is described by an independent 1st-order SDE in the OU process, the time series $\{V_n\}_{n\in \mathbb N}$ is described by an AR(1) process. On the contrary, the evolution of the $x$ variables is non Markovian and expressed, at the continuous level, via a generalized Langevin equation. Consequently, the time series $\{\bar V_n\}_{n\in \mathbb N}$ inherits a nonzero MA order, ending in an ARMA(1,1). Nonetheless, we may ask whether it is possible to describe it with an \emph{effective} AR(1) process, which would correspond to an effective AR(2) process for the $\{X_n\}_{n\in \mathbb N}$ series.

Let us write a putative AR(1) model for the series of reconstructed velocities:
\begin{equation}
	\bar V_n - (1-\alpha) \bar V_{n-1} = \sigma \epsilon_n, 
	\label{AR1-effective}
\end{equation}
%where $L$ is the aforementioned lag operator, 
where $\epsilon_n\sim\mathcal N(0,1)$ I.I.D. and $\alpha$, $\sigma$ are parameters to fix. The goal is to find an effective memoryless discrete model for $\{\bar V_n\}_{n\in \mathbb N}$ that reproduces correctly the sufficient statistics used by Bayesian and non-Bayesian parametric inference approaches based on the exploitation of \emph{local} dynamical information. The common characteristic of these approaches is being derived from a Taylor-It\^o expansion in the small $\tau$ limit; hence they just exploit short time information to learn the laws governing the evolution of the system. This information is typically carried by the first few elements of the autocovariance of the time series. 

In the case of the integrated Ornstein Uhlenbeck process, a sufficient statistics corresponds to the set $\mathcal S_1 = \left\{\Exp {\bar V_n^2},\Exp {\bar V_n \bar V_{n+1}}\right\}$, i.e. the self-correlations of the reconstructed velocities at equal time and at a distance of one time step. %, or, equivalently, to the set $\mathcal S_2  = \left\{\Exp {\bar X_n^2},\Exp {\bar X_n \bar X_{n+1}}, \Exp {\bar X_n \bar X_{n+2}}\right\}$. 
The choice of the sufficient statistics is not unique, but this results to be particularly convenient for its possible interpretation in the context of maximum caliber approaches \cite{LeePresse}. 

%Notice that this means it's the same as using a max caliber approach taking as constrained observables the self-correlation of the observed process at equal time, one time step and two time step.

We impose on these observables the two following \emph{consistency} conditions:
\begin{enumerate}
\item[i.] $\bar V_n$ follows a Maxwell Boltzmann distribution with temperature $T$. Since the only parameter of the distribution is the variance, this condition corresponds to equipartition ($k_B=1$):
\begin{equation}
	\Exp{\bar V_n^2} = T.
	\label{equip}
\end{equation}
\item[ii.] The relation between the reconstructed acceleration $\bar A_n = (\bar V_{n+1}-\bar V_n)/\tau$ and the reconstructed velocity $\bar V_n$ is the one we can exactly compute for the integrated Ornstein-Uhlenbeck process: 
\begin{equation}
\Exp{\bar A_n\vert \bar V_n} \mathop{\simeq}_{\tau\to 0} -\frac{2}{3}\eta \bar V_n.
\label{ped-relation}
\end{equation}
A detailed derivation is in \cite{Pedersen}. From this relation we immediately derive the condition to impose on the observables of interest:
\begin{equation}
	\Exp{\bar V_{n+1}\bar V_n} = \left(1-\frac{2}{3}\eta\tau\right) \Exp{\bar V_n^2}.
	\label{ped}
\end{equation}
%The covariance of the random increment of Eq.~\eqref{AR1-effective} matches the diagonal entries of the covariance of the consistent scheme of order 3/2:
%\begin{equation}
%	\Exp{r_n^2} = \sigma^2\Exp{\epsilon_n^2} = \frac{2}{3}2T\eta\tau.
%\end{equation}
%This operation corresponds to applying a mask on the covariance matrix wich cancels color and only retains its diagonal entries.
\end{enumerate}
The self-correlation function $\Exp{\bar V_n \bar V_{n+k}}$ of an AR(1) process of the form of Eq.~\eqref{AR1-effective} is explicitly known:
\begin{equation}
	\Exp{\bar V_n \bar V_{n+k}} = \frac{(1-\alpha)^{|k|}\sigma^2}{1-(1-\alpha)^2}.
	\label{self-corr}
\end{equation}
Taking its value at $k=1$ and using Eq.~\eqref{equip} in Eq.~\eqref{ped} yields the expected result $\alpha=(2/3) \eta\tau$. Computing the self-correlation of the reconstructed velocities at $k=0$ and imposing equipartition, we set the value of $\sigma$:
\begin{equation}
	\sigma^2 = T \left[1-(1-\alpha)^2\right] \mathop{\simeq}_{\tau\to0}  2T\alpha.
	\label{Einstein}
\end{equation}
This is the celebrated Einstein relation.

In conclusion, it is possible to describe the sequence of measurements of an integrated OU process as an effective AR(2) series with a rescaled damping coefficient $\eta' = (2/3)\eta$. Replacing the obtained values for $\alpha$ and $\sigma$ in Eq.~\eqref{AR1-effective} and using the definition of $\bar V_n$, the generative model reads:
\begin{equation}
X_n - \left(2-\frac{2}{3}\eta\tau\right) X_{n-1} + \left(1-\frac{2}{3}\eta\tau\right) X_{n-1} = \left(\frac{4}{3}T\eta\tau^3\right)^{1/2}\epsilon_n.
\end{equation}
This result is intuitive and could have been grossly derived by imposing the Einstein relation (which in fact comes from Eq.~\eqref{equip} alone), and applying a mask to the covariance matrix of random increments which only selects the main diagonal and cancels color, thus implying $\sigma^2=\frac{2}{3}2T\eta\tau$ (to replace Eq.~\eqref{ped}).

Of course, this effective discretization can only be used at the scale of $\tau$: it gives, by construction, consistent maximum likelihood estimators when applied to inference problems, but cannot be iterated in simulations to reproduce the process on longer scales. Because of the convergence of Euler-Maruyama integration algorithm, the simulated process would be the damped Langevin model with a damping coefficient equal to $\eta'$.

Although the derivation is based on the linear and integrated nature of the process, which allows us to work with the reconstructed velocity series $\{\bar V_n\}_{n\in \mathbb N}$, we argue that the same results hold in the presence of linear forces, where the second fluctuation-dissipation theorem holds \cite{Kubo}. In addition, we conjecture that the same rescaling of the $\eta$ coefficient can be adopted as a ``shortcut to Markovianity" even for non-Gaussian equilibrium processes, described by generalizations of the Langevin equations \eqref{eq-xv-1}--\eqref{eq-xv-2}, where the elastic force is replaced by $f(x)=-\nabla U(x)$. 
This conjecture is inspired by numerical results. Applying, for instance, Euler-based inference schemes to a simulated time series with $f(x) = - kx - \lambda x^3$, one obtains a damping coefficient $\eta$ rescaled of a factor 2/3, while the parameter estimator for the temperature of the heat bath is consistent. Results are shown in Fig.~\ref{fig:anharmonic}. The remaining parameters modulating the force term are wrongly reconstructed using the naive Euler discretization, because dynamical information of higher order in $\tau$ (not accessible through the Euler scheme) is required to disentangle the contributions of the different terms in the polynomial force.  %Details about the adopted inference procedure are explained in the following section.
 
We hope that this consideration can help simplifying the dynamical inference procedure in those experimental contexts where the observed phenomena are modelled via effective damped equilibrium processes, and inertial degrees of freedom are the only ones to be directly accessible. 

\begin{figure}
\includegraphics[width=.32\columnwidth]{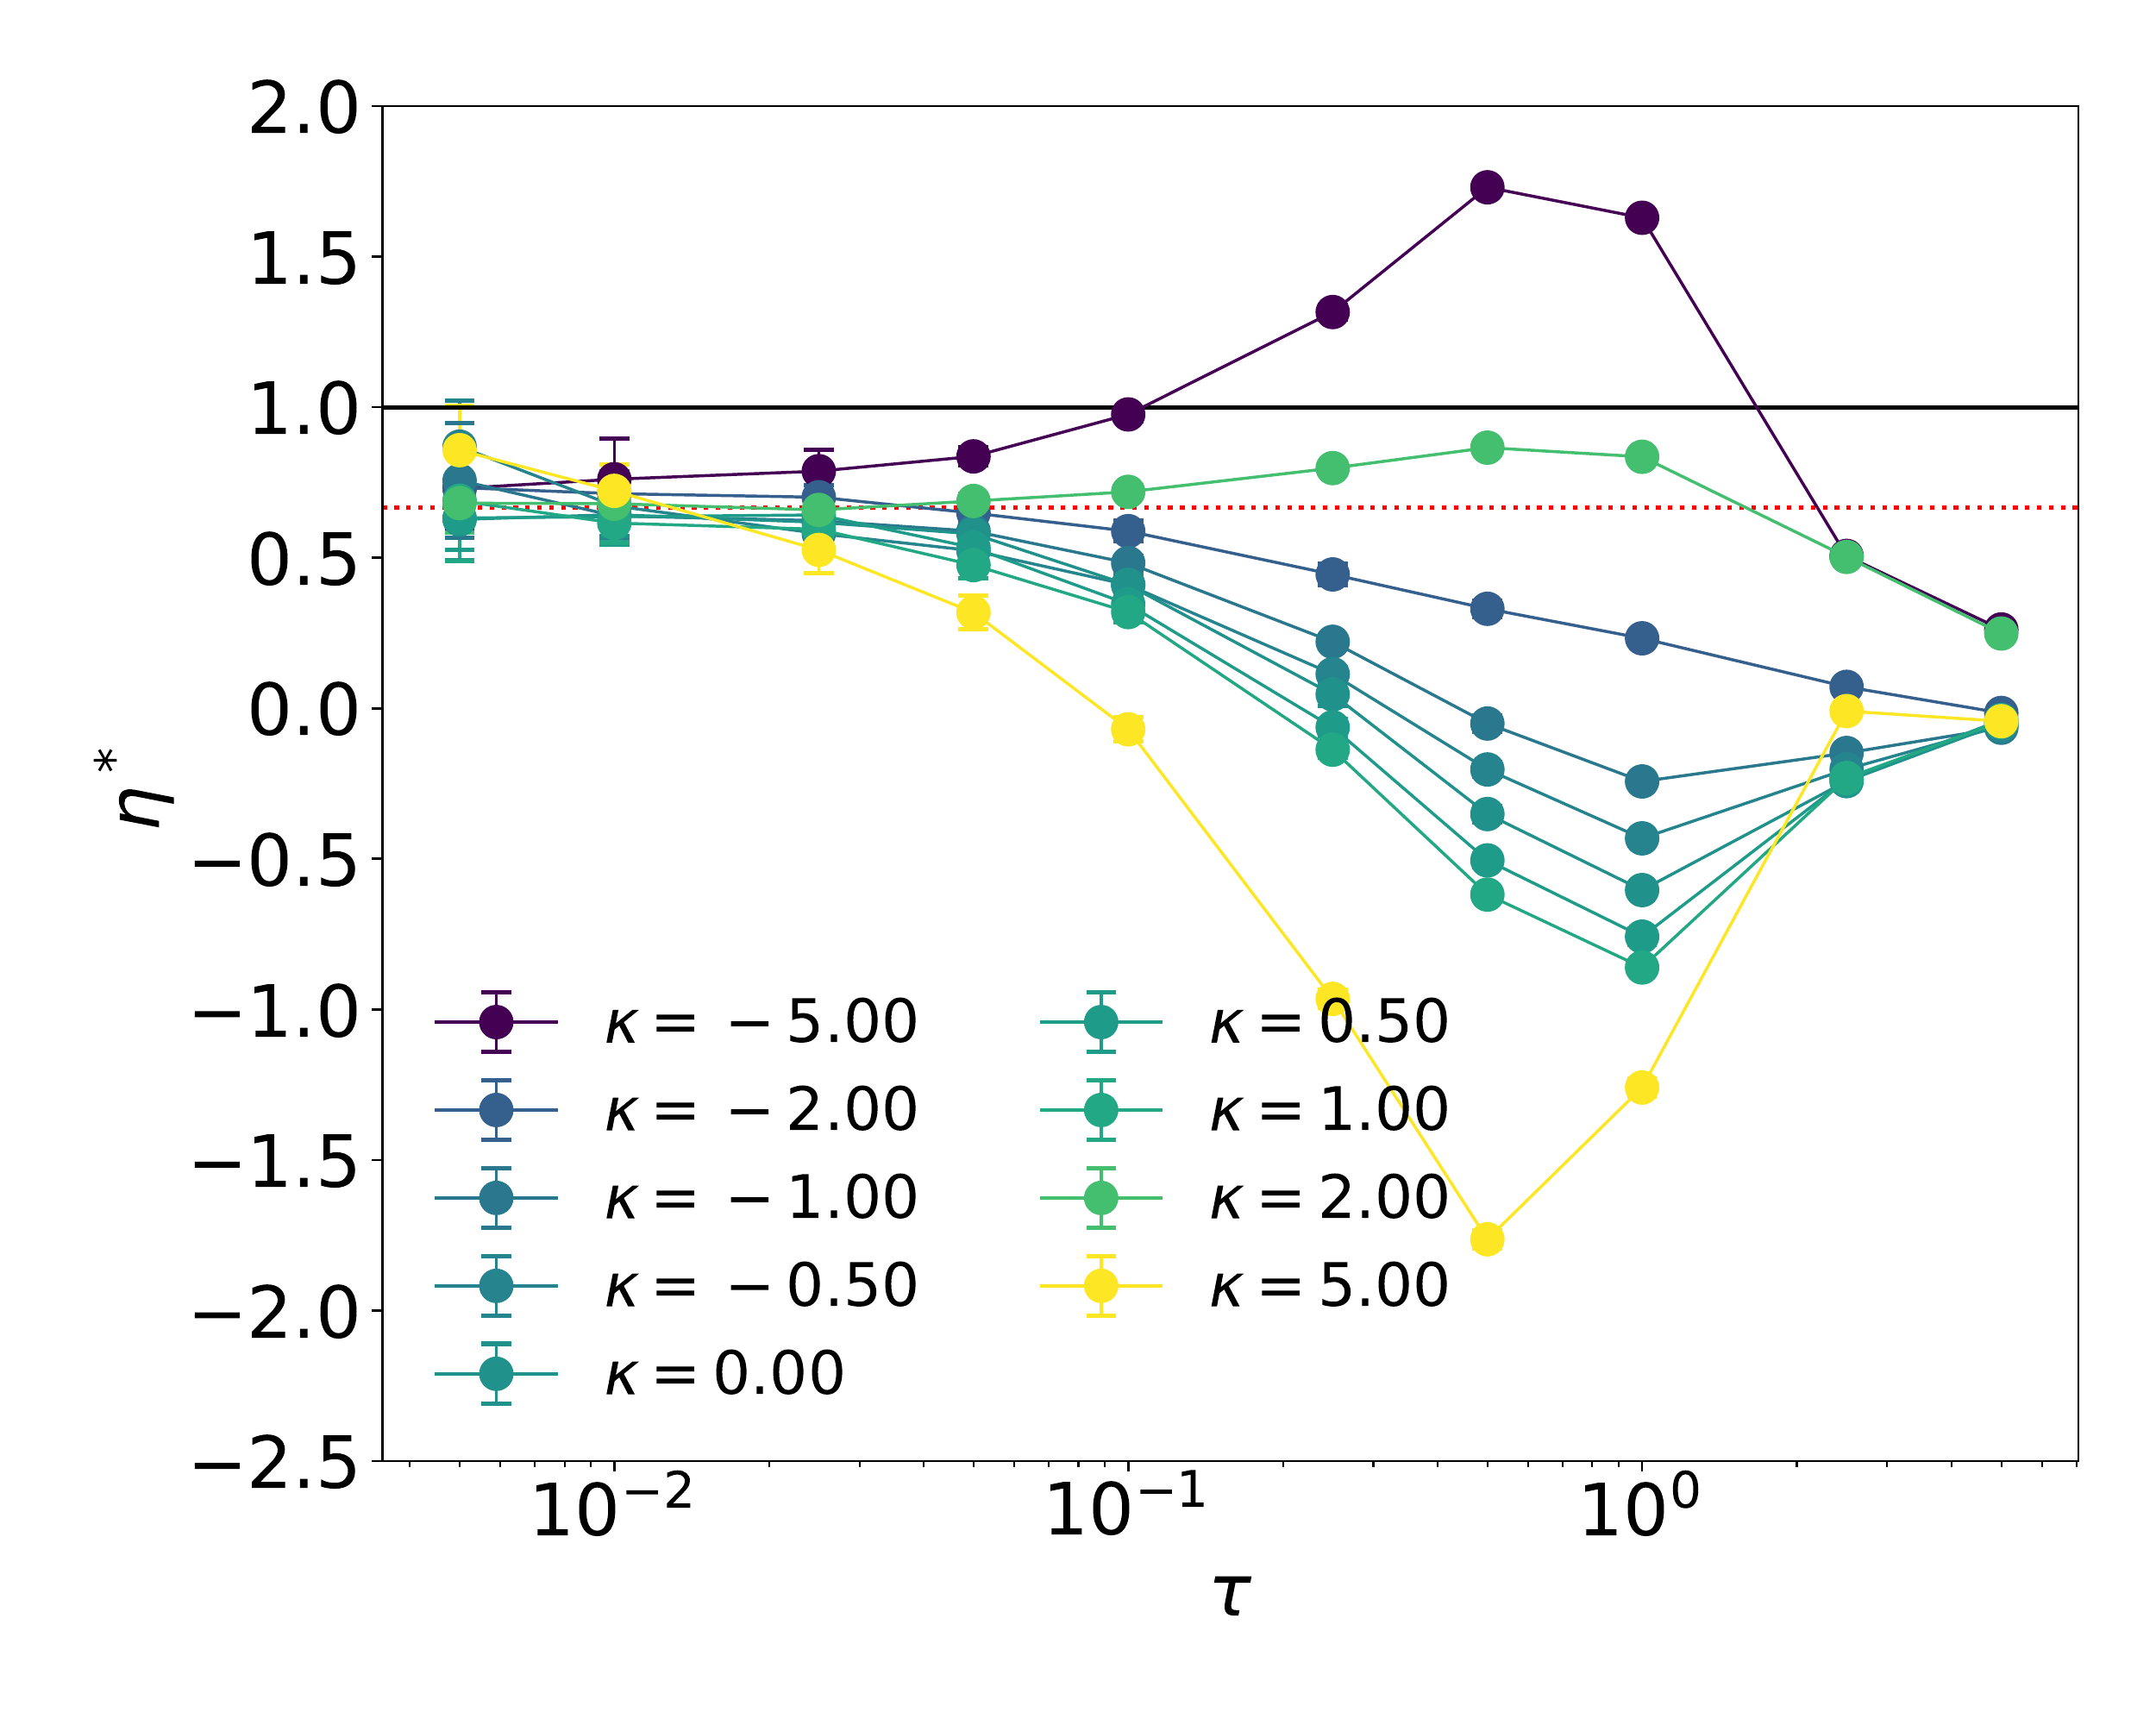}\llap{  \parbox[b]{1cm}{a\\\rule{0ex}{1.55in}}}
\includegraphics[width=.32\columnwidth]{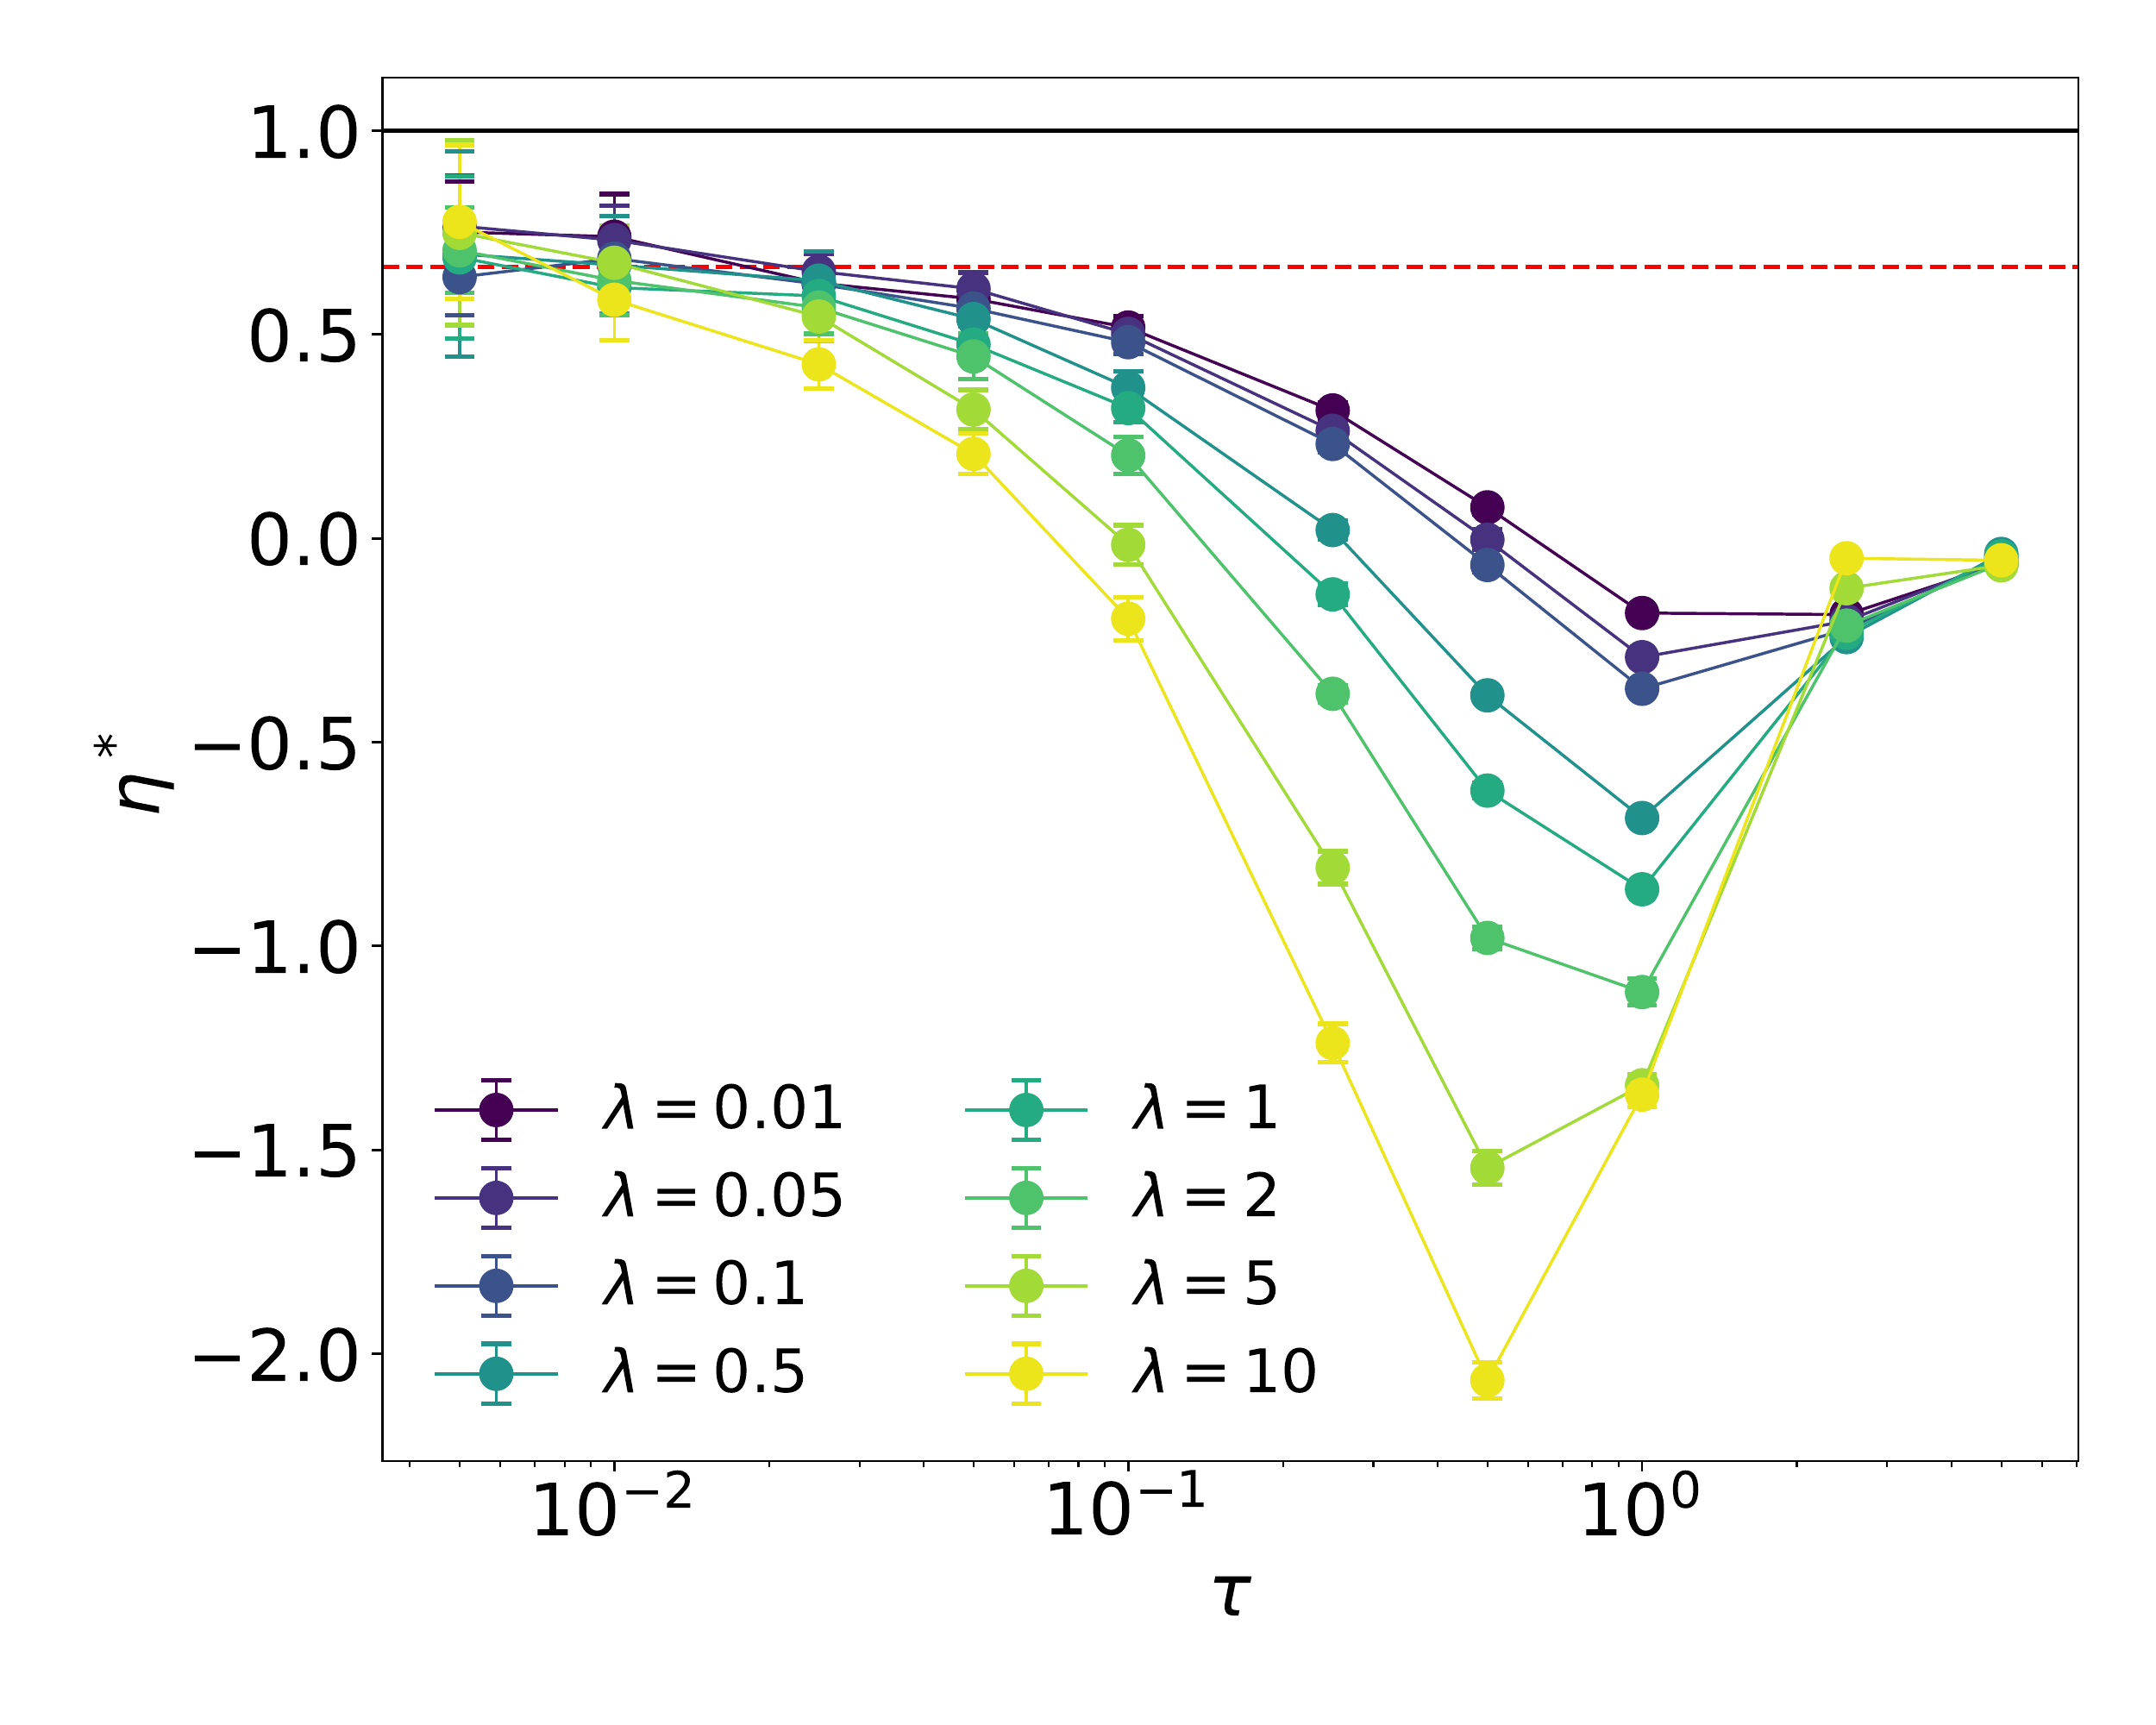}\llap{  \parbox[b]{1cm}{b\\\rule{0ex}{1.55in}}}
\includegraphics[width=.32\columnwidth]{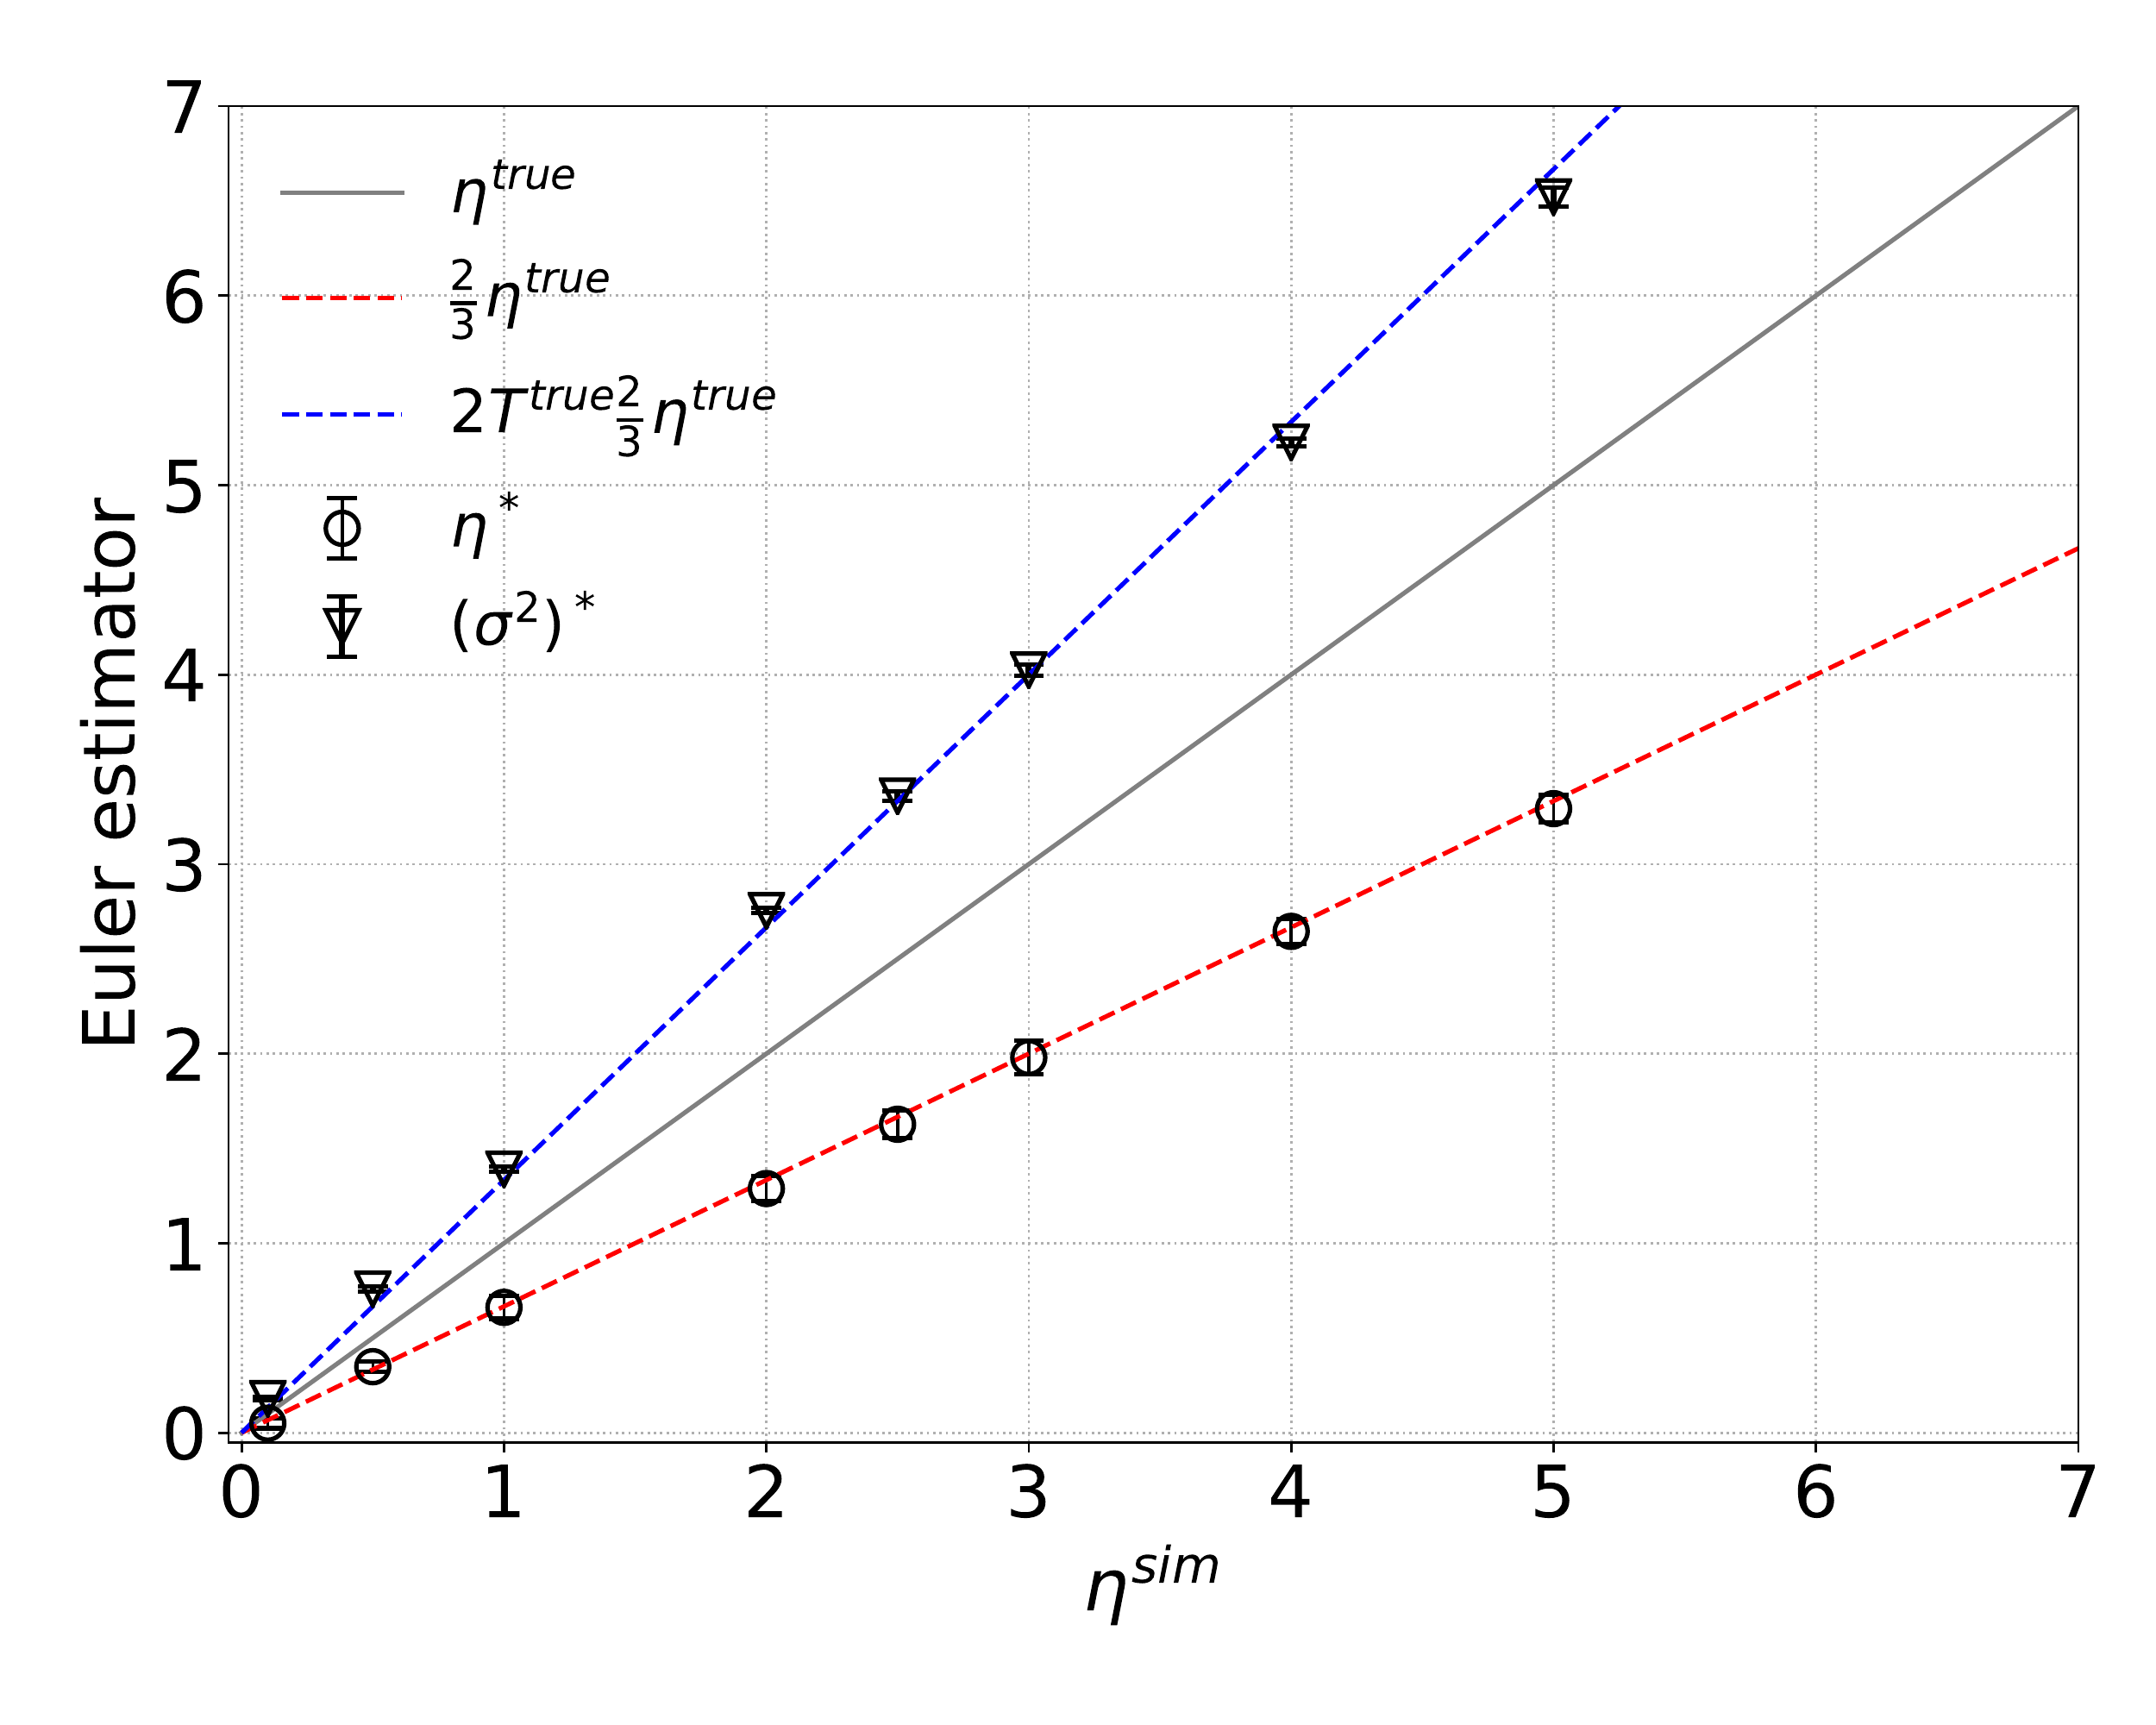}\llap{  \parbox[b]{1cm}{c\\\rule{0ex}{1.55in}}}
\caption{Inconsistent Maximum Likelihood estimators for the damping coefficient $\eta$ of a Brownian process in a symmetric quartic potential: $dx = vdt$; $dv = -\eta v dt - \kappa x dt -\lambda x^3 dt + \sigma dW$. These estimators are obtained by applying the Euler discretization for the derivation of an approximate likelihood, which removes color and yields an incorrect Markovian description of the system. Nonetheless, the effect on the estimator $\eta^*$ is just a $2/3$ rescaling factor (in the $\tau\to0$ limit). The same rescaling affects the diffusion coefficient $\sigma^2=2T\eta$; hence the equilibrium temperature $T$ is correctly estimated. The parameters used to generate the time series analyzed in the figures above are: (a) $\lambda=1,\, \eta=1$; (b) $\kappa=1,\, \eta=1$; (c) $\kappa=-1, \, \lambda=1$. Estimators $\kappa^*$ and $\lambda^*$ obtained with the same Euler-based procedure are inconsistent.}
\label{fig:anharmonic}
\end{figure}
